# Supplementary material for: Out-of-distributional risk bounds for neural operators with applications to the Helmholtz equation
Source: arXiv:2301.11509 source file (2023-07-04)
Supplement: Supplementary file 1 [file 3.tex]

% -----------------------------------------------------------------------
\section{Numerical results of the different neural network architectures}
\label{experiments}
%\subsection{Architectures' parameters}\label{exp:architectures}
% -----------------------------------------------------------------------

We evaluate the performance of the different 
architectures using the datasets described in 
\cref{Euler_equation}, that is, in the context 
of acoustic wave propagation.
For the two experiments we have introduced 
in \cref{Euler_equation}, we detail the parameters 
and training used for the different architecture, 
and show the reconstruction.

% ---------------------------------------------------------------------------
\subsection{Experiment 1}
% ---------------------------------------------------------------------------

% ----------------------------------------------------------
\subsubsection{Parameters of the architectures and training}
% ----------------------------------------------------------

For Experiment 1 presented \cref{experiment1,figure:cp-GRF:experiment1},
the parameters in the four versions of Neural Operators tested are 
given \cref{table:hyperparam:experiment1}. 

\begin{table}[h!]
\centering
\scalebox{0.85}{\begin{tabular}{l|c|c|c|c|}
\cline{2-5}
                                                                                            & \multicolumn{1}{l|}{\textbf{FNO}}                                     & \multicolumn{1}{l|}{\textbf{$\MNO$}}                                   & \multicolumn{1}{l|}{\textbf{($\FNONeXt$)v1}}                  & \multicolumn{1}{l|}{\textbf{($\FNONeXt$)v2}}                                                                   \\ \hline
\multicolumn{1}{|l|}{\textbf{Modes}}      & 12  & 12 & 12 & $[12, 12, 12, 12]$      \\ \hline
\multicolumn{1}{|l|}{\textbf{Layers}}     & 4   & 4  & 4  & $[3,3,9,3]$             \\ \hline
\multicolumn{1}{|l|}{\textbf{Features}}   & 36  & 36 & 36 & $[36, 36, 36, 36]$      \\ \hline
\multicolumn{1}{|l|}{\textbf{Activation}} & GELU& GELU & GELU & GELU                \\ \hline
\multicolumn{1}{|l|}{\textbf{\begin{tabular}[c]{@{}l@{}}Positional                  \\ 
encoder\end{tabular}}} & \begin{tabular}[c]{@{}c@{}}with grid on \\ $[-1,1]^2$\end{tabular}   
& with grid on  $[-1,1]^2$  & with grid on  $[-1,1]^2$   & with grid on  $[-1,1]^2$ \\ \hline
\multicolumn{1}{|l|}{\textbf{Lifting}}   & \begin{tabular}[c]{@{}c@{}}MLP(ReLU):    \\ $3\to 18\to 36$
\end{tabular}  & \begin{tabular}[c]{@{}c@{}}MLP(ReLU):\\ $3\to 18\to 36$\end{tabular} 
               & \begin{tabular}[c]{@{}c@{}}MLP(ReLU):\\ $3\to 18\to 36$\end{tabular} 
               & \begin{tabular}[c]{@{}c@{}}MLP(ReLU):\\ $3\to 18\to 36$\end{tabular} 
               \\ \hline
\multicolumn{1}{|l|}{\textbf{Projection}}                                                   & \begin{tabular}[c]{@{}c@{}}MLP (ReLU):\\ $36\to 18\to 1$\end{tabular} & \begin{tabular}[c]{@{}c@{}}MLP(ReLU):\\ $36\to 18\to 1$\end{tabular} & \begin{tabular}[c]{@{}c@{}}MLP(ReLU):\\ $36\to 18\to 1$\end{tabular} & \begin{tabular}[c]{@{}c@{}}MLP(ReLU):\\ $36\to 18\to 1$\end{tabular} \\ \hline
\multicolumn{1}{|l|}{\textbf{Dropout}}                                                      & No                                                                    & No                                                                   & No                                                                   & 0.1                                                                  \\ \hline
\multicolumn{1}{|l|}{\textbf{Drop Path}}                                                    & No                                                                    & No                                                                   & No                                                                   & 0.3                                                                  \\ \hline
\end{tabular}}

\caption{\textbf{Architectures' parameters used with the dataset of 
         Experiment 1 (\cref{experiment1,figure:cp-GRF:experiment1})}. 
  All architectures use the same hyperparameters, except
  for ($\FNONeXt$) version 2. 
  Following \citet[2.2 Macrodesign]{liu2022convnet}, 
  we have the combination layers=$[3,3,9,3]$ ($18$ layers), modes=$[12, 12, 16, 14]$,  and
  $\#$features $[30, 30, 32, 38]$. Interpreted as follows: $3$ consecutive 
  layers with $12$ modes, and feature space of $30$, and so on.}
\label{table:hyperparam:experiment1}
\end{table}

From the results in Experiment 1 \cref{experiment1} the following can be concluded.
\begin{enumerate}
    \item We do not notice \textit{advantage of using dropout} for $4$ layers architectures.
    \item  We find advantage of using dropout and stochastic depth, whenever the network becomes deep, and overfitting naturally occurs. Besides, we empirically find a major effectiveness of stochastic depth (drop path) \citep{huang2016deep}. 
    \item The stochastic depth in the ($\FNONeXt$) version $2$ increases linearly from $0$ in the first layer, to $0.3$ in the last.
    \item The MLP (local part) of the last three architectures, see Figures~\ref{fig:MFNO} and \ref{fig:FNO+epsilon} for visualization, is chosen to be a small MLP. \\
    Mapping: $$\#\mathrm{feature} \to 4(\#\mathrm{feature}) \to \#\mathrm{feature}.$$ 
    
    We keep the inverse bottleneck tradition in Transformers, and  \citet[2.4]{liu2022convnet}, popularized in \citet{sandler2018mobilenetv2}.
\end{enumerate}

\subsubsection{Training of Experiment 1}
The training uses the following components:
\begin{enumerate}
    \item For all the architectures we use Adam Optimizer \citep{kingma2014adam}, with an initial learning rate $10^{-3}$, with a StepLR scheduler with parameters: step size=$80$, and a multiplicative factor of learning rate decay of $\gamma=0.5$.
    \item The number of epochs is chosen to $100$ for the first $3$ architectures (FNO, $\MNO$ and ($\FNONeXt$) version $1$). For the last, ($\FNONeXt$) version $2$, it is extended to $200$ (the main purpose is to push the architecture as much as possible, and follows some of the training recipes in Transformers and ConvNeXt).
    \item In all the architectures, we use a small $\ell_2$-weight regularizer with parameter $10^{-5}$.
    \item The training is implemented with $25 000$ of $30000$, the testing is make with $5000$.
\end{enumerate}

% ---------------------------------------------
\subsubsection{Results of Experiment 1}
\label{exp:results}
% ---------------------------------------------

Following training using couples made up of wave 
speeds and pressure fields described \cref{Euler_equation},
the objective of the network is to predict a
pressure field given a GRF realization of wave speed.
In \cref{figure:results-experiment1}, we show the results
for three realizations of wave speeds in the context of 
Experiment~1. The norms of the relative difference with
the reference solution (obtained from the discretization
of the PDE) for 6 realizations are given \cref{table:experiment1:l2error}.

% ---------------------------
\setlength{\modelwidth} {4cm}
\setlength{\modelheight}{4cm}
\graphicspath{{Figures/results_experiment1/}}
% ---------------------------
\begin{figure}[ht!]\centering
\input{Figures/results_experiment1/skeleton_oneline_model1} 

\input{Figures/results_experiment1/skeleton_oneline_model2} 

\input{Figures/results_experiment1/skeleton_oneline_model3}

\vspace*{-0.50em}

    \caption{\small{ 
            %\textbf{(Real part) of the pressure field reconstructed by
             Pressure field reconstructed for 
             Experiment 1 (\cref{experiment1,figure:cp-GRF:experiment1}) 
             with the different architectures for three test-cases. 
             \textit{First column} shows independent GRF realization of the wave
             speed (see \cref{Euler_equation}).  
             \textit{Second column} shows the solution of the wave PDE
             obtained with software \texttt{hawen} \citep{faucher2021hawen}, 
             which we consider as the \emph{reference solution},
             see \cref{Euler_equation}. 
             \textit{Other columns} show the approximated reconstruction 
             using the different architectures:
             \textit{FNO}, see \citet{kovachki2021neural}; 
             $\multiplicative$ structure ($\MFNO$, see~\cref{MNO}); 
             and the solutions provided by $\FNONeXt$, \cref{FNO+epsilon}.
             In each case, we show the real part of the pressure field, and 
             the relative error with the reference solution using a logarithmic
             scale.
             }}

\label{figure:results-experiment1}
\end{figure}

\begin{table}[!ht]
\centering
\captionsetup{format=plain,labelfont=bf,font=small} % Customize caption style
\begin{tabular}{@{}lllll@{}}
\toprule
\textbf{Models} & \textbf{FNO} & \textbf{$\MFNO$} & \textbf{($\FNONeXt$)v1} & \textbf{($\FNONeXt$)v2} \\ 
\midrule
 1 & $0.4030$     & $0.2788$      & $0.2419$                       & $0.0869$                       \\ 
 2 & $0.4155$     & $0.2703$      & $0.2477$                       & $0.0993$                       \\ 
 3 & $0.4548$     & $0.2980$      & $0.2414$                       & $0.0902$                       \\ 
 4 & $0.4396$     & $0.2855$      & $0.2453$                       & $0.0810$                       \\ 
 5 & $0.4325$     & $0.2768$      & $0.2442$                       & $0.0849$                       \\ 
 6 & $0.4301$     & $0.2800$      & $0.2538$                       & $0.0877$                       \\ 
\bottomrule
\end{tabular}
\caption{Norm of the relative $\mathrm{L}_2$-norm for Experiment 1 \cref{experiment1}. Multiple realization of the trained networs with different random seed. Each row represent a different realization, and the values corresponds to the test loss of the architectures after training. The visualization of the table is presented in the main section of the paper, \cref{fig:boxplot}.}
\label{table:experiment1:l2error}
\end{table}

We see that the reconstructions using FNO are the 
least accurate and do not fully capture the interference
patterns of waves, in all three cases pictures in 
\cref{figure:results-experiment2_12Hz}.
The results obtained with architectures ($\FNONeXt$)v1
and $\MFNO$ are relatively closed, even though 
($\FNONeXt$)v1 appears slightly more accurate in terms
of relative error. 
Architecture ($\FNONeXt$)v2, that uses more layers,
is the most accurate with relative error of about one order 
of magnitude less than the others.

%%%%%%%%%%%%%%%%%%%%%%%%%%%%%%%%%%%%%%%%%%%%%%%%%%%%%%%%%%%%%%%%%%%%%%%%%%%
%Comparison experiment 1
%%%%%%%%%%%%%%%%%%%%%%%%%%%%%%%%%%%%%%%%%%%%%%%%%%%%%%%%%%%%%%%%%%%%%%%%%%%

\subsubsection{Comparison of the Experiment 1 (multiple random initializations)}

We randomly initialize the architectures, and we generate the equivalent diagram of Figure~\ref{fig:boxplot} at $\omega/(2\pi) = 7, 15$ Hz. The results are consistent with the behavior in Figure~\ref{fig:boxplot}, throughout multiple realizations of the networks' parameters and training paths. It should be noticed that the behavior is more pronounced at higher frequencies. Showing the advantages of the network's modifications.

\begin{figure}[!ht]
    \centering
    \includegraphics[scale= 0.5]{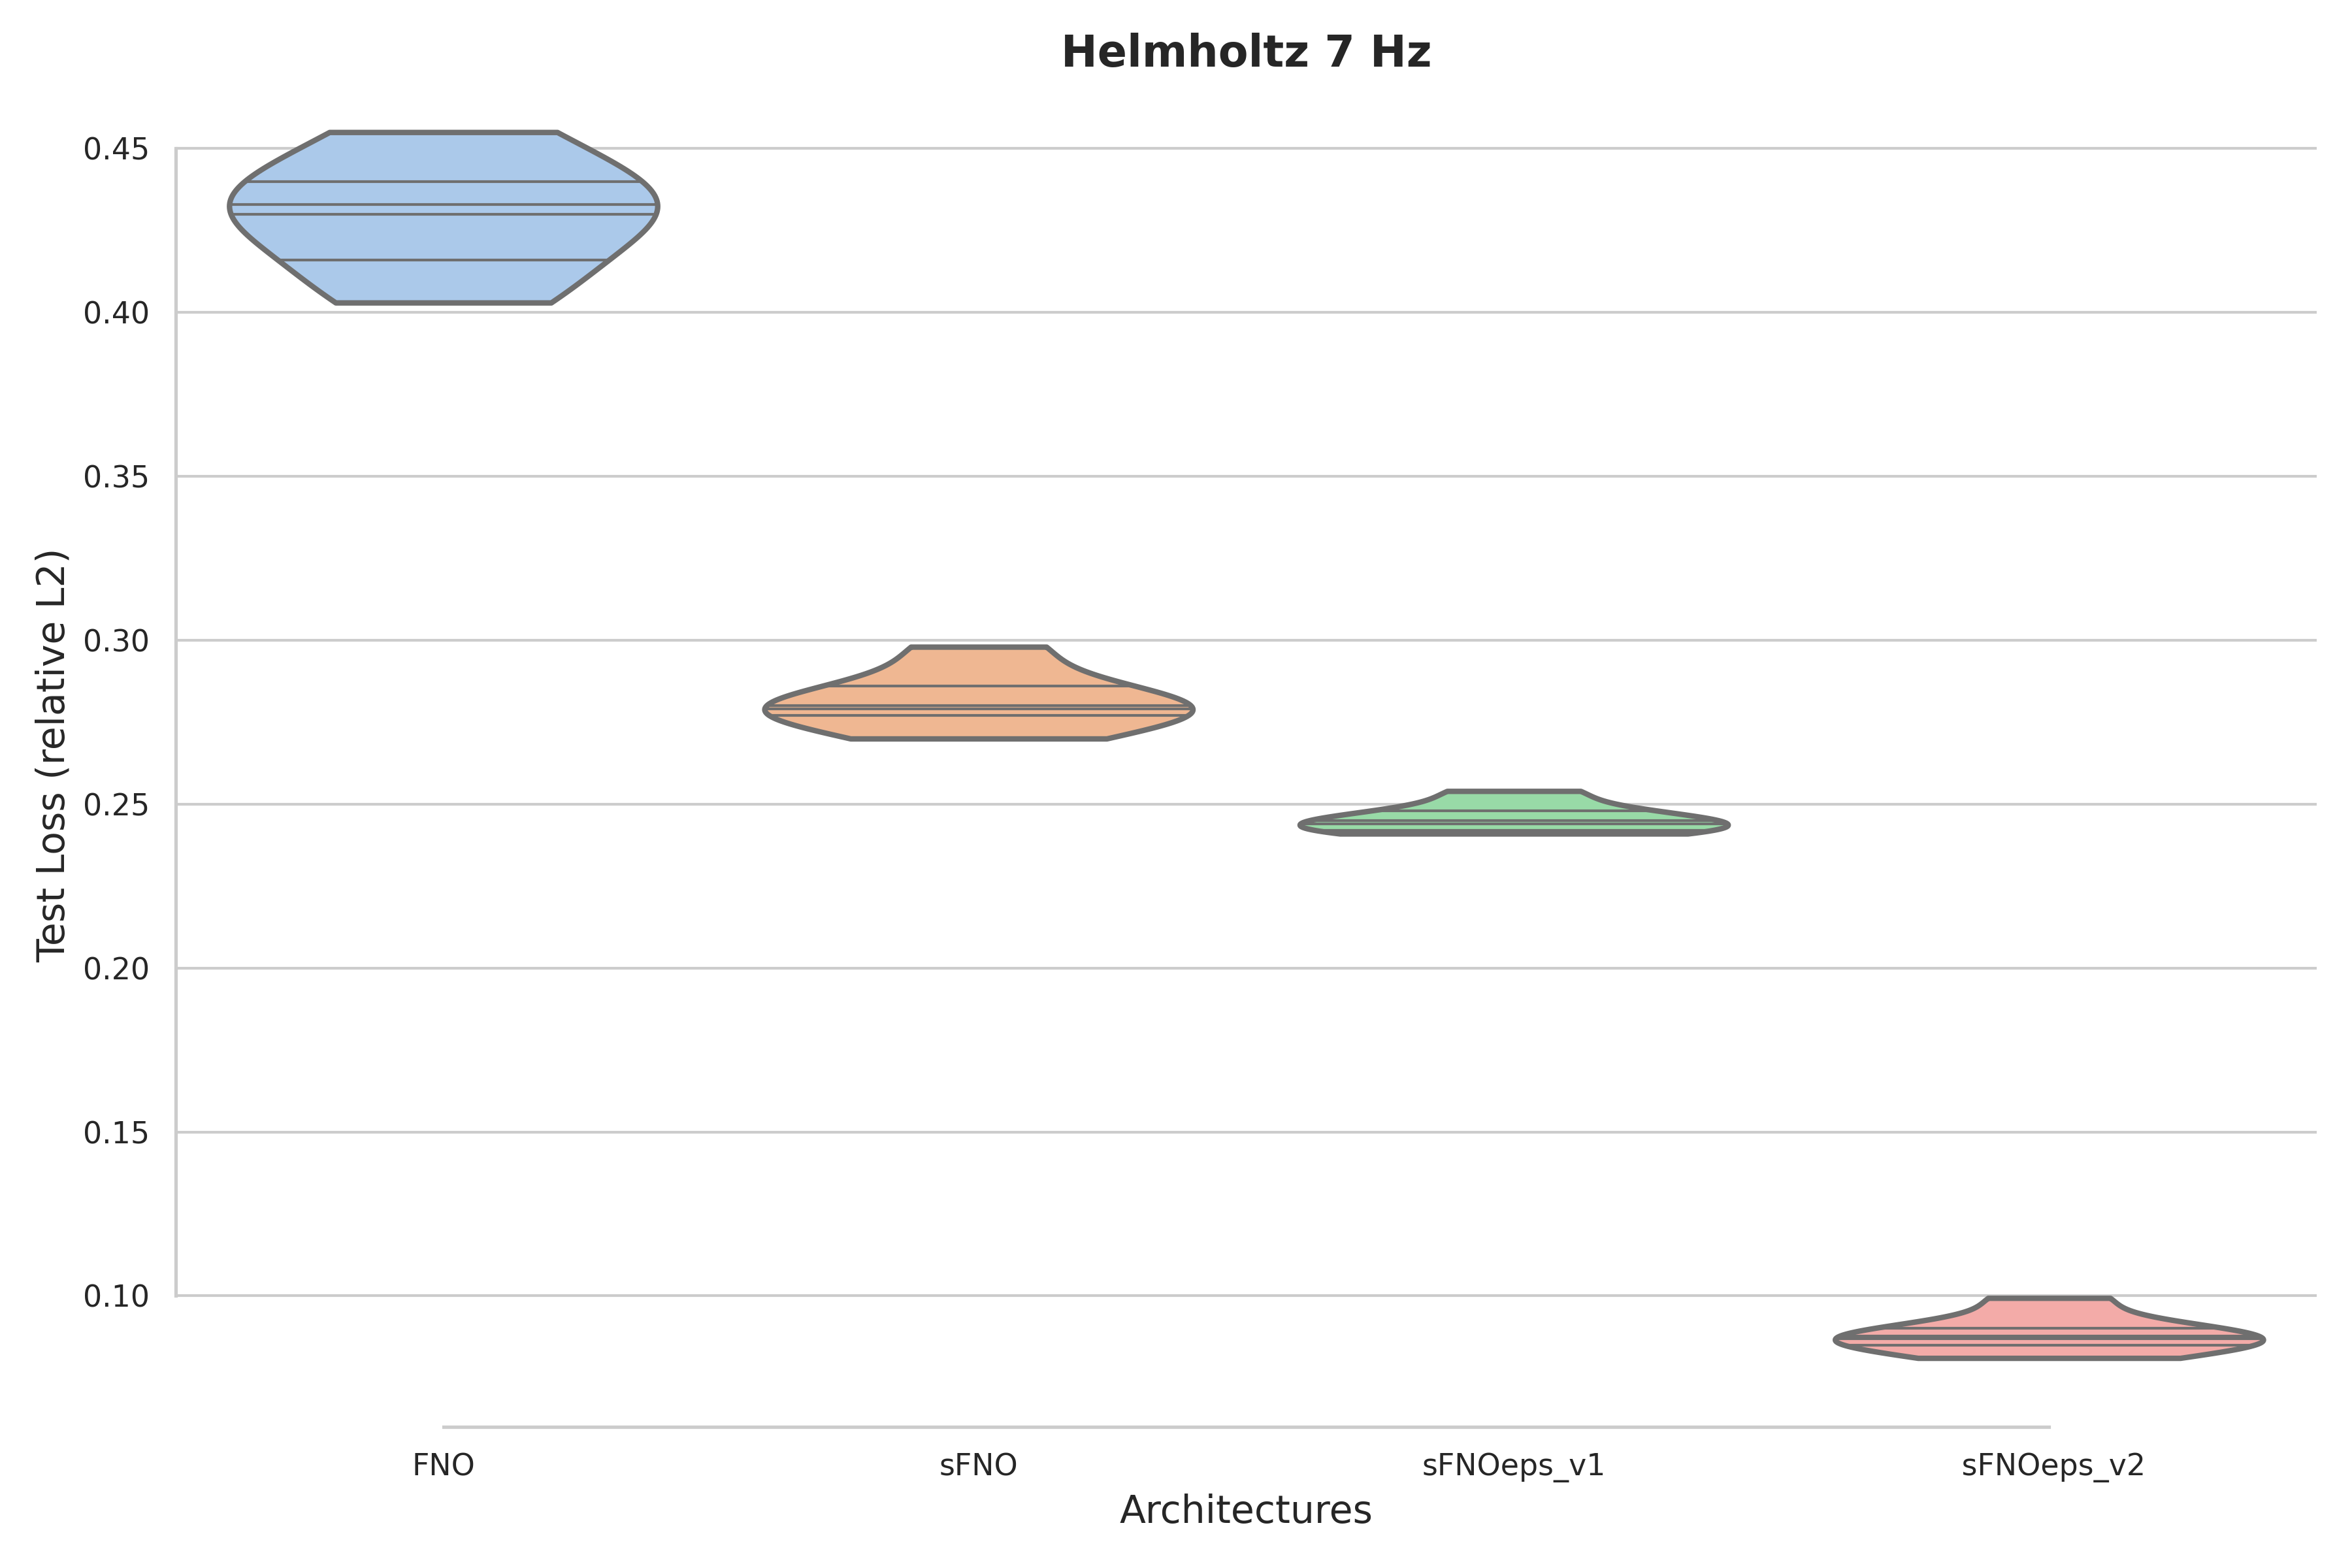}
    \caption{\small{\textbf{Comparison of test-loss for the Experiment~1 of \cref{Euler_equation} ($\omega/(2\pi) = 7$ Hz). Each architecture is trained $9$ times, the relative $\Lp$-loss, $\|\Gcal^{\mathrm{ref}} - \Gcal^{\mathrm{approx}}\|_{\Lp}/ \|\Gcal^{\mathrm{ref}}\|_{\Lp}$, on the test set is shown in the diagram.}}}
    \label{fig:boxplot_12}
\end{figure}

% ---------------------------------------------------------------------------
\subsection{Experiment 2}\label{exp:results2}
% ---------------------------------------------------------------------------

% ----------------------------------------------------------
\subsubsection{Parameters of the architectures and training}
% ----------------------------------------------------------

For Experiment 2 presented \cref{experiment2,figure:cp-GRF:experiment2},
the parameters in the four versions of Neural Operators tested are 
given \cref{table:hyperparam:experiment2}. 
In this experiment, we further compare two frequencies 
for the wave propagation with $\omega/(2\pi)$ set to 12 
and 15 \si{\Hz} for \cref{eq:Euler}.

\begin{table}[ht!]
\centering
\scalebox{0.85}{\begin{tabular}{l|c|c|c|c|}
\cline{2-5}
                                                                                            & \multicolumn{1}{l|}{\textbf{FNO}}                                     & \multicolumn{1}{l|}{\textbf{$\MFNO$}}                                   & \multicolumn{1}{l|}{\textbf{($\FNONeXt$)v1}}                  & \multicolumn{1}{l|}{\textbf{($\FNONeXt$)v2}}                  \\ \hline
\multicolumn{1}{|l|}{\textbf{Modes}}                                                        & 12                                                                    & 12                                                                   & 12                                                                   & $[12, 12, 16, 14]$                                                   \\ \hline
\multicolumn{1}{|l|}{\textbf{Layers}}                                                       & 4                                                                     & 4                                                                    & 4                                                                    & $[3,3,9,3]$                                                          \\ \hline
\multicolumn{1}{|l|}{\textbf{Features}}                                                     & 36                                                                    & 36                                                                   & 36                                                                   & $[30, 30, 32, 38]$                                                   \\ \hline
\multicolumn{1}{|l|}{\textbf{Activation}}                                                   & GELU                                                                  & GELU                                                                 & GELU                                                                 & GELU                                                                 \\ \hline
\multicolumn{1}{|l|}{\textbf{\begin{tabular}[c]{@{}l@{}}Positional\\ encoder\end{tabular}}} & \begin{tabular}[c]{@{}c@{}}with grid on \\ $[-1,1]^2$\end{tabular}    & with grid on  $[-1,1]^2$                                             & with grid on  $[-1,1]^2$                                             & with grid on  $[-1,1]^2$                                             \\ \hline
\multicolumn{1}{|l|}{\textbf{Lifting}}                                                      & \begin{tabular}[c]{@{}c@{}}MLP(ReLU):\\ $3\to 18\to 36$\end{tabular}  & \begin{tabular}[c]{@{}c@{}}MLP(ReLU):\\ $3\to 18\to 36$\end{tabular} & \begin{tabular}[c]{@{}c@{}}MLP(ReLU):\\ $3\to 18\to 36$\end{tabular} & \begin{tabular}[c]{@{}c@{}}MLP(ReLU):\\ $3\to 18\to 36$\end{tabular} \\ \hline
\multicolumn{1}{|l|}{\textbf{Projection}}                                                   & \begin{tabular}[c]{@{}c@{}}MLP (Id):\\ $36\to 1$\end{tabular} & \begin{tabular}[c]{@{}c@{}}MLP(Id):\\ $36\to 2$\end{tabular} & \begin{tabular}[c]{@{}c@{}}MLP(Id):\\ $36\to 2$\end{tabular} & \begin{tabular}[c]{@{}c@{}}MLP(Id):\\ $36\to 2$\end{tabular} \\ \hline
\multicolumn{1}{|l|}{\textbf{Dropout}}                                                      & No                                                                    & No                                                                   & No                                                                   & 0.1                                                                  \\ \hline
\multicolumn{1}{|l|}{\textbf{Drop Path}}                                                    & No                                                                    & No                                                                   & No                                                                   & 0.3                                                                  \\ \hline
\end{tabular}}

\caption{\textbf{Architectures' parameters 12 Hz and 15 Hz}. The only architecture that differs is ($\FNONeXt$) version $2$ similarly than Experiment 1. Furthermore, there are two differences with respect to \cref{table:hyperparam:experiment2}, (a) the networks recovered both real, and imaginary part of the pressure field in the time-harmonic wave equation, i.e., the output is a vector field in $\mathbb{R}^2$ which can be associated with $\mathbb{C}$, and (b) the projection operator is simplified by a linear layer instead of a MLP to speed up the training process.}
\label{table:hyperparam:experiment2}
\end{table}

%%%%%%%%%%%%%%%%%%%%%%%%%%%%%%%%%%%%%%%%%%%%%%%%%%%%%%%%%%%%%%%%%%
\subsubsection{Training of Experiment 2}
The training uses the following components:
\begin{enumerate}
    \item For all the architectures we use Adam Optimizer \citep{kingma2014adam}, with an initial learning rate $10^{-3}$, with a StepLR scheduler with parameters: step size=$80$, and a multiplicative factor of learning rate decay of $\gamma=0.5$.
    \item The number of epochs is chosen to $100$ for the first $3$ architectures (FNO, $\MFNO$ and $\FNONeXt$) version $1$). For the last, ($\FNONeXt$) version $2$, it is extended to $200$ (the main purpose is to push the architecture as much as possible, and follows some of the training recipies in Transformers and ConvNeXt).
    \item In all the architectures, we use a small $\ell_2$-weight regularizer with parameter $10^{-5}$.
    \item The training is implemented with $25 000$ of $50000$, validation with $5000$ generated samples, the testing is make with $25000$.
\end{enumerate}

% ---------------------------------------------
\subsubsection{Results of Experiment 2}
% ---------------------------------------------

In \cref{figure:results-experiment2_12Hz,figure:results-experiment2_15Hz}, 
we show the results for three realization of wave speeds in the context of 
Experiment~2, respectively for frequency $\omega/(2\pi)$ set to 12 and 
15 \si{\Hz}.

% ---------------------------
\setlength{\modelwidth} {4cm}
\setlength{\modelheight}{4cm}
\graphicspath{{Figures/results_experiment2_12Hz/}}
% ---------------------------
\begin{figure}[ht!]\centering
\input{Figures/results_experiment2_12Hz/skeleton_oneline_model1b} 
\vspace*{2em}

\input{Figures/results_experiment2_12Hz/skeleton_oneline_model2b}
    \caption{\small{ 
            %\textbf{(Real part) of the pressure field reconstructed by
             Pressure field (12 \si{\Hz}) reconstructed for 
             Experiment 2 (\cref{experiment2,figure:cp-GRF:experiment2}) 
             at frequency \num{12} \si{\Hz}
             with the different architectures for two GRF 
             realizations of the wave speed. 
             \textit{Left column} shows independent GRF realization of the wave
             speed (see \cref{Euler_equation}).  
             \textit{Second column} shows the real and imaginary parts
             of the pressure field solution to the wave PDE at frequency
             12 \si{\Hz}, 
             obtained with software \texttt{hawen} \citep{faucher2021hawen}, 
             which we consider as the \emph{reference solution},
             see \cref{Euler_equation}. 
             \textit{Other columns} show the approximated reconstructions 
             using the different architectures:
             \textit{FNO}, see \citet{kovachki2021neural}; 
             $\multiplicative$ structure ($\MFNO$, see~\cref{MNO}); 
             and the solutions provided by $\FNONeXt$, \cref{FNO+epsilon}.
             In each case, we show the real and imaginary 
             parts of the pressure fields, and 
             the relative error with the reference 
             solution on a logarithmic scale.
             }}
\label{figure:results-experiment2_12Hz}
\end{figure}

% ---------------------------
\setlength{\modelwidth} {4cm}
\setlength{\modelheight}{4cm}
\graphicspath{{Figures/results_experiment2_15Hz/}}
% ---------------------------
\begin{figure}[ht!]\centering
\input{Figures/results_experiment2_15Hz/skeleton_oneline_model2b} 
\vspace*{2em}

\input{Figures/results_experiment2_15Hz/skeleton_oneline_model1b}

    \caption{\small{ 
            %\textbf{(Real part) of the pressure field reconstructed by
             Pressure field (15 \si{\Hz}) reconstructed for 
             Experiment 2 (\cref{experiment2,figure:cp-GRF:experiment2}) 
             at frequency \num{15} \si{\Hz}
             with the different architectures for two GRF 
             realizations of the wave speed. 
             \textit{Left column} shows independent GRF realization of the wave
             speed (see \cref{Euler_equation}).  
             \textit{Second column} shows the real and imaginary parts
             of the pressure field solution to the wave PDE at frequency
             15 \si{\Hz}, 
             obtained with software \texttt{hawen} \citep{faucher2021hawen}, 
             which we consider as the \emph{reference solution},
             see \cref{Euler_equation}. 
             \textit{Other columns} show the approximated reconstructions 
             using the different architectures:
             \textit{FNO}, see \citet{kovachki2021neural}; 
             $\multiplicative$ structure ($\MFNO$, see~\cref{MNO}); 
             and the solutions provided by $\FNONeXt$, \cref{FNO+epsilon}.
             In each case, we show the real and imaginary 
             parts of the pressure fields, and 
             the relative error with the reference 
             solution on a logarithmic scale.
             }}

\label{figure:results-experiment2_15Hz}
\end{figure}
We see that the best reconstructions are obtained using 
architecture ($\FNONeXt$)v2, which is expected as
it uses multiple layers. The reconstruction with FNO is less accurate than the other, 
and we observe that ($\FNONeXt$)v1 is slightly more 
accurate than the architecture $\MNO$ in all cases.
Comparing the frequencies, it appears that higher frequencies
(15 \si{\Hz} in \cref{figure:results-experiment2_15Hz} compared
to 12 \si{\Hz} in \cref{figure:results-experiment2_12Hz}) are 
slightly harder to reconstruct. This can be explained as the 
wavelength becomes smaller, hence more oscillations and features
have to be anticipated by the networks.
The results of Experiments 2 are 
totally consistent with Experiment~1 of \cref{figure:results-experiment1}.
Consequently, we see that the approach is robust
with respect to the change in the the position of 
the source, the size of the domain, variation of wave speeds,
and change of frequencies.

%%%%%%%%%%%%%%%%%%%%%%%%%%%%%%%%%%%%%%%%%%%%%%%%%%%%%%%%%%%%%%%%%%%%%%%%%%%
%Comparison experiment 2
%%%%%%%%%%%%%%%%%%%%%%%%%%%%%%%%%%%%%%%%%%%%%%%%%%%%%%%%%%%%%%%%%%%%%%%%%%%
\subsubsection{Comparison of the Experiment 2 (multiple random initializations)}
We randomly initialize the architectures, and we generate the equivalent diagram of Figure~\ref{fig:boxplot} at higher frequencies $\omega/(2\pi) = 12$ Hz. The results are consistent with the behavior in Figure~\ref{fig:boxplot}, throughout multiple realizations of the networks' parameters and training paths. 
\begin{figure}[!htb]
    \centering
    \includegraphics[scale= 0.5]{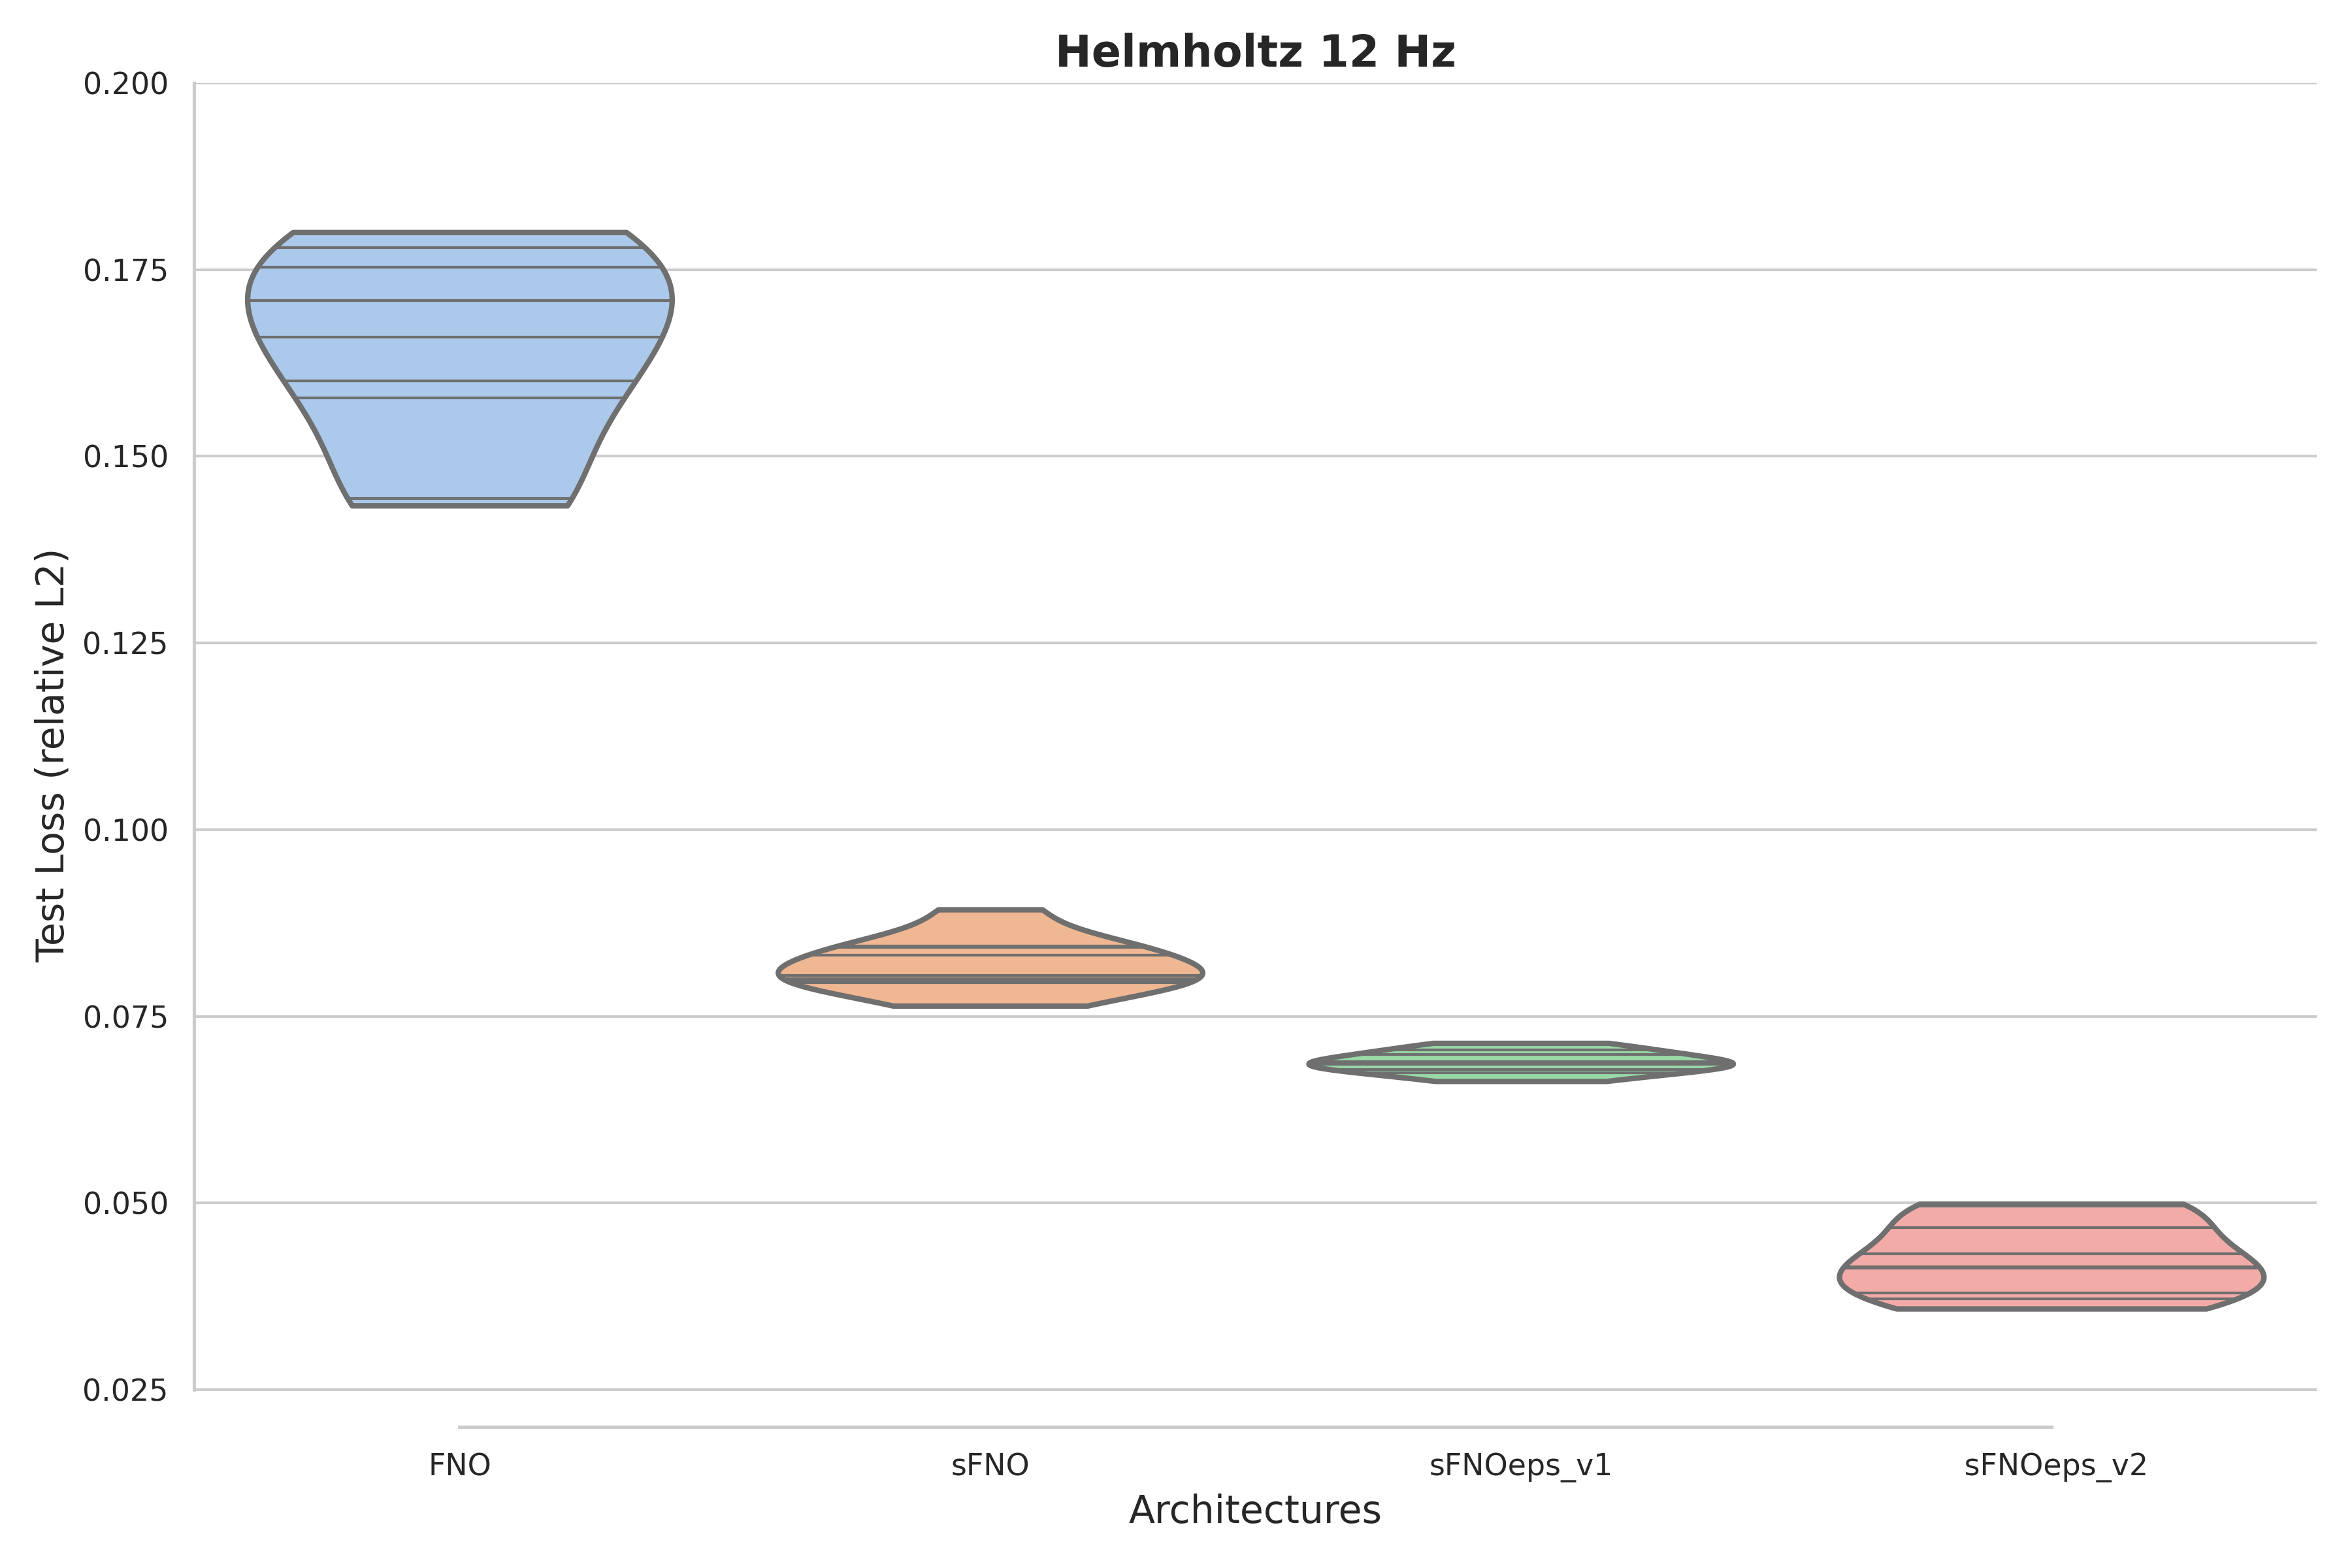}
    \caption{\small{Comparison of test-loss for the Experiment~2 of \cref{Euler_equation} ($\omega/(2\pi) = 12$ Hz). Each architecture is trained $9$ times, the relative $\Lp$-loss, $\|\Gcal^{\mathrm{ref}} - \Gcal^{\mathrm{approx}}\|_{\Lp}/ \|\Gcal^{\mathrm{ref}}\|_{\Lp}$, on the test set is shown in the diagram.}}
    \label{fig:boxplot_12}
\end{figure}

\newpage
\subsection{Parameter size of the models}
In this section we review the parameter size of all the models.

\iffalse{
\begin{table}[ht!]
\centering
\begin{tabular}{|l|l|l|l|l|}
\hline
\# Param & FNO (Baseline) & sFNO & sFNO+eps v1 & sFNO+eps v2 \\ \hline
 Lifting & 756 & 756 & 756 & 3.5k\\ \hline
Proj & 685 & 685 & 685 & 3.5k \\ \hline
Operator NN & 1.5M & 1.5M & 1.5M & 8.1M \\ \hline

\end{tabular}
\caption{Summary of parameters of each network, following the specifications in \cref{table:hyperparam:experiment1}, and \cref{table:hyperparam:experiment2}}
\label{table:Models_Size}
\end{table}}\fi 

\begin{table}[ht!]
\centering
\captionsetup{format=plain,labelfont=bf,font=small} % Customize caption style
\begin{tabular}{@{}lllll@{}}
\toprule
\# Param & FNO (Baseline) & sFNO & sFNO+eps v1 & sFNO+eps v2 \\
\midrule
Lifting & 756 & 756 & 756 & 3.5k \\
Proj & 685 & 685 & 685 & 3.5k \\
Operator NN & 1.5M & 1.5M & 1.5M & 8.1M \\
\bottomrule
\end{tabular}
\caption{Summary of parameters of each network, following the specifications in Table 1 and Table 2}
\label{table:Models_Size}
\end{table}

\subsection{PDE benchmarks} \label{benchmarks_appendix}
The data is obtained from \citet{li2020fourier}. We do not normalize the data, nor using the pointwise Gaussian normalization from the \texttt{utils.py} script from \cite{FNO:2022:Online} as originally presented, given that is not possible to establish for longer data set as the time-harmonic case \cref{dataset:Helmholtz}. The parameters are the same as \cref{table:hyperparam:experiment1} and 
\cref{table:hyperparam:experiment2}.
%%%%%%%%%%%%%%%%%%%%%%%%%%%%%%%%%%%%%%%%%%%%%%%%%%%%%%%%%
%Darcy Flow
%%%%%%%%%%%%%%%%%%%%%%%%%%%%%%%%%%%%%%%%%%%%%%%%%%%%%%%%%
\subsubsection{Darcy Flow}\label{appendix:Darcy}
We follow the same procedure as it is described in \cite{li2020fourier}.
\begin{table}[ht!]
\centering
\captionsetup{format=plain,labelfont=bf,font=small} % Customize caption style
\begin{tabular}{@{}lllll@{}}
\toprule
Models & FNO (Baseline) & sFNO & sFNO+eps v1 & sFNO+eps v2 \\ 
\midrule
 1& 0.017649 & 0.0161063 & 0.015746 & 0.013619 \\ 
 2& 0.018546 & 0.015157 & 0.015534 & 0.014038 \\ 
 3& 0.017843 & 0.018314 & 0.016719 & 0.013507 \\ 
 4& 0.018624 & 0.014651 & 0.015104 & 0.015567 \\ 
 5& 0.019044 & 0.015499 & 0.015570 & 0.012848 \\ 
\bottomrule
\end{tabular}
\caption{Summary of the empirical error of all the architectures with respect to Darcy flow. We randomly initialize the architecture $5$ to have a consistent analysis of the test loss.}
\label{table:DarcyFlow}
\end{table}
\subsubsection{Navier-Stokes}\label{appendix:NS}
%%%%%%%%%%%%%%%%%%%%%%%%%%%%%%%%%%%%%%%%%%%%%%%%%%%%%%%%%
%NS
%%%%%%%%%%%%%%%%%%%%%%%%%%%%%%%%%%%%%%%%%%%%%%%%%%%%%%%%%
Similarly as before we do not use any normalization in the input's data, and we tested the architectures with viscosity $\nu = 10^{-4}$ using the $10000$ samples provided. We divided them into $7000$ for training and $3000$ for testing. 
\begin{table}[ht!]
\centering
\captionsetup{format=plain,labelfont=bf,font=small} % Customize caption style
\begin{tabular}{@{}lllll@{}}
\hline
\toprule
Models & FNO (Baseline) & sFNO & sFNO+eps v1 & sFNO+eps v2 \\ 
\midrule
 1& 0.2645 & 0.2164 & 0.2094 & 0.1861 \\ 
 2& 0.2630 & 0.2118 & 0.2064 & 0.1869 \\ 
 3& 0.2638 & 0.2163 & 0.2092 & 0.1854 \\ 
\bottomrule
\end{tabular}
\caption{Summary of the empirical error of all the architectures with respect to the version of Navier-Stokes presented in \citet{li2020fourier}. We randomly initialize the architecture $3$ to have a consistent analysis of the test loss.}
\label{table:NavierStokes}
\end{table}

\subsection{Ablation}\label{appendix:ablation}
In some extent the gradual analysis of architectures investigate the ablation. That is, if the skip connection is removed, sNO+$\varepsilon$ v1 reduces to sNO. Likewise, sNO+$\varepsilon$ v2, with $\mathbb{P}(X = 1) = 1$ reduces to sNO+$\varepsilon$ v1. Hence, the ablation analysis is implicity set in the body of the paper wiht exception of the ResNet version of NOs \cite{you2022learning}. Regarding sNO and NO, the analysis of the Radamacher complexity \cref{sNO_GEB} suffices to show the differences in the re-structured of the architecture, and \cref{sNOeps_GEB}. The parameters presented in \cref{table:hyperparam:experiment1}, and \cref{table:hyperparam:experiment2} are the same for all the networks not included ($\FNONeXt$)v2, we change the modes to $12$, feature to $36$, and training to $100$ epochs to have a constant analysis among parameters.

\subsubsection{time-harmonic wave equation at $12$Hz: GeLU activation}
\begin{table}[!ht]
\centering
\captionsetup{format=plain,labelfont=bf,font=small} % Customize caption style
\begin{tabular}{@{}llllll@{}}
\toprule
Models & Baseline FNO & ResNet FNO & sFNO & sFNO+eps v1 & sFNO+eps v2  \\
\midrule
 1 & 0.1708 & 0.0895 & 0.0805 & 0.0678 & 0.0414  \\
 2 & 0.1578 & 0.0807 & 0.0800 & 0.0663 & 0.0413  \\
 3 & 0.1659 & 0.0902 & 0.0795 & 0.0674 & 0.0371  \\
\bottomrule
\end{tabular}
\caption{Model Performance Comparison time-harmonic wave equation at $12$Hz. The error is the relative test loss.}
\end{table}

\subsubsection{time-harmonic wave equation at $15$Hz: GeLU activation}
\begin{table}[!ht]
\centering
\captionsetup{format=plain,labelfont=bf,font=small} % Customize caption style
\begin{tabular}{@{}llllll@{}}
\toprule
Models & Baseline FNO & ResNet FNO & sFNO & sFNO+eps v1 & sFNO+eps v2  \\
\midrule
 1 & 0.1724 & 0.1131 & 0.1275 & 0.0980 & 0.0623  \\
 2 & 0.1744 & 0.1249 & 0.1131 & 0.0982 & 0.0624  \\
 3 & 0.1757 & 0.1202 & 0.1267 & 0.1049 & 0.0689  \\
\bottomrule
\end{tabular}
\caption{Model Performance Comparison time-harmonic wave equation at $15$Hz. The error is the relative test loss.}
\end{table}

We observed that among our multiple trained models the skip connection by itself improve the performance of the model, which it agrees with the analysis obtained by \citet{you2022learning}. Last but not least, our model benefits from the presence of the MLP after the linear integral operator.

\subsubsection{time-harmonic wave equation at $15$Hz: ReLU activation}
\begin{table}[!ht]
\centering
\captionsetup{format=plain,labelfont=bf,font=small} % Customize caption style
\begin{tabular}{@{}llllll@{}}
\toprule
Models & Baseline FNO & ResNet FNO & sFNO & sFNO+eps v1 & sFNO+eps v2  \\
\midrule
 1 & 0.1968 & 0.1787 & 8 &  &   \\
 2 & 0.2086 & 0.1544 &  & &  \\
 3 & 0.2370 & 0.1517 &  &  &   \\
\bottomrule
\end{tabular}
\caption{Model Performance Comparison time-harmonic wave equation at $15$Hz. The error is the relative test loss using ReLU activation.}
\end{table}

\subsubsection{time-harmonic wave equation at $15$Hz: Identity activation}
\begin{table}[!ht]
\centering
\captionsetup{format=plain,labelfont=bf,font=small} % Customize caption style
\begin{tabular}{@{}llllll@{}}
\toprule
Models & Baseline FNO & ResNet FNO & sFNO & sFNO+eps v1 & sFNO+eps v2  \\
\midrule
 1 & 0.8730 & 0.2198 & & &   \\
 2 & 0.8806 & 0.2500 &  &  &  \\
 3 & 0.8850 & 0.2122 &  &  &  \\
\bottomrule
\end{tabular}
\caption{Model Performance Comparison time-harmonic wave equation at $15$Hz. The error is the relative test loss using Identity activation.}
\end{table}
