# Supplementary material for: Out-of-distributional risk bounds for neural operators with applications to the Helmholtz equation
Source: arXiv:2301.11509 source file (2023-07-04)
Supplement: Supplementary file 2 [file 4.tex]

\subsection{Visualization of the loss landscape of all the architectures (Experiment 1 data).} \label{visualization_appendix}

The significant performance differences observed between the considered architectures prompted us to investigate their respective loss landscapes. For that purpose, we used the loss landscape visualization method proposed by \citet{li2018visualizing} and its open-source implementation~\citet{visualloss:2019:Online}. This approach's basic idea consists of computing the principal components of the weights associated with each model obtained during training. In particular, the first two principal components span a two-dimensional domain that can be sampled to yield a loss surface centered around the optimized model. While this transformation amounts to a dramatic linear dimensionality reduction, it has been shown to offer valuable insight into important qualitative differences between architectures~\citep{li2018visualizing}.

\cref{fig:landscapes} shows two-dimensional and three-dimensional views of the loss landscapes corresponding to the FNO, $\MFNO$, and $\FNONeXt$ architectures. Note that all visualizations use identical scaling factors and color scales to facilitate comparisons. Similarly, the level sets correspond to the same set of loss values.

\begin{figure}[h!]
\center 
\includegraphics[width=0.99\linewidth]{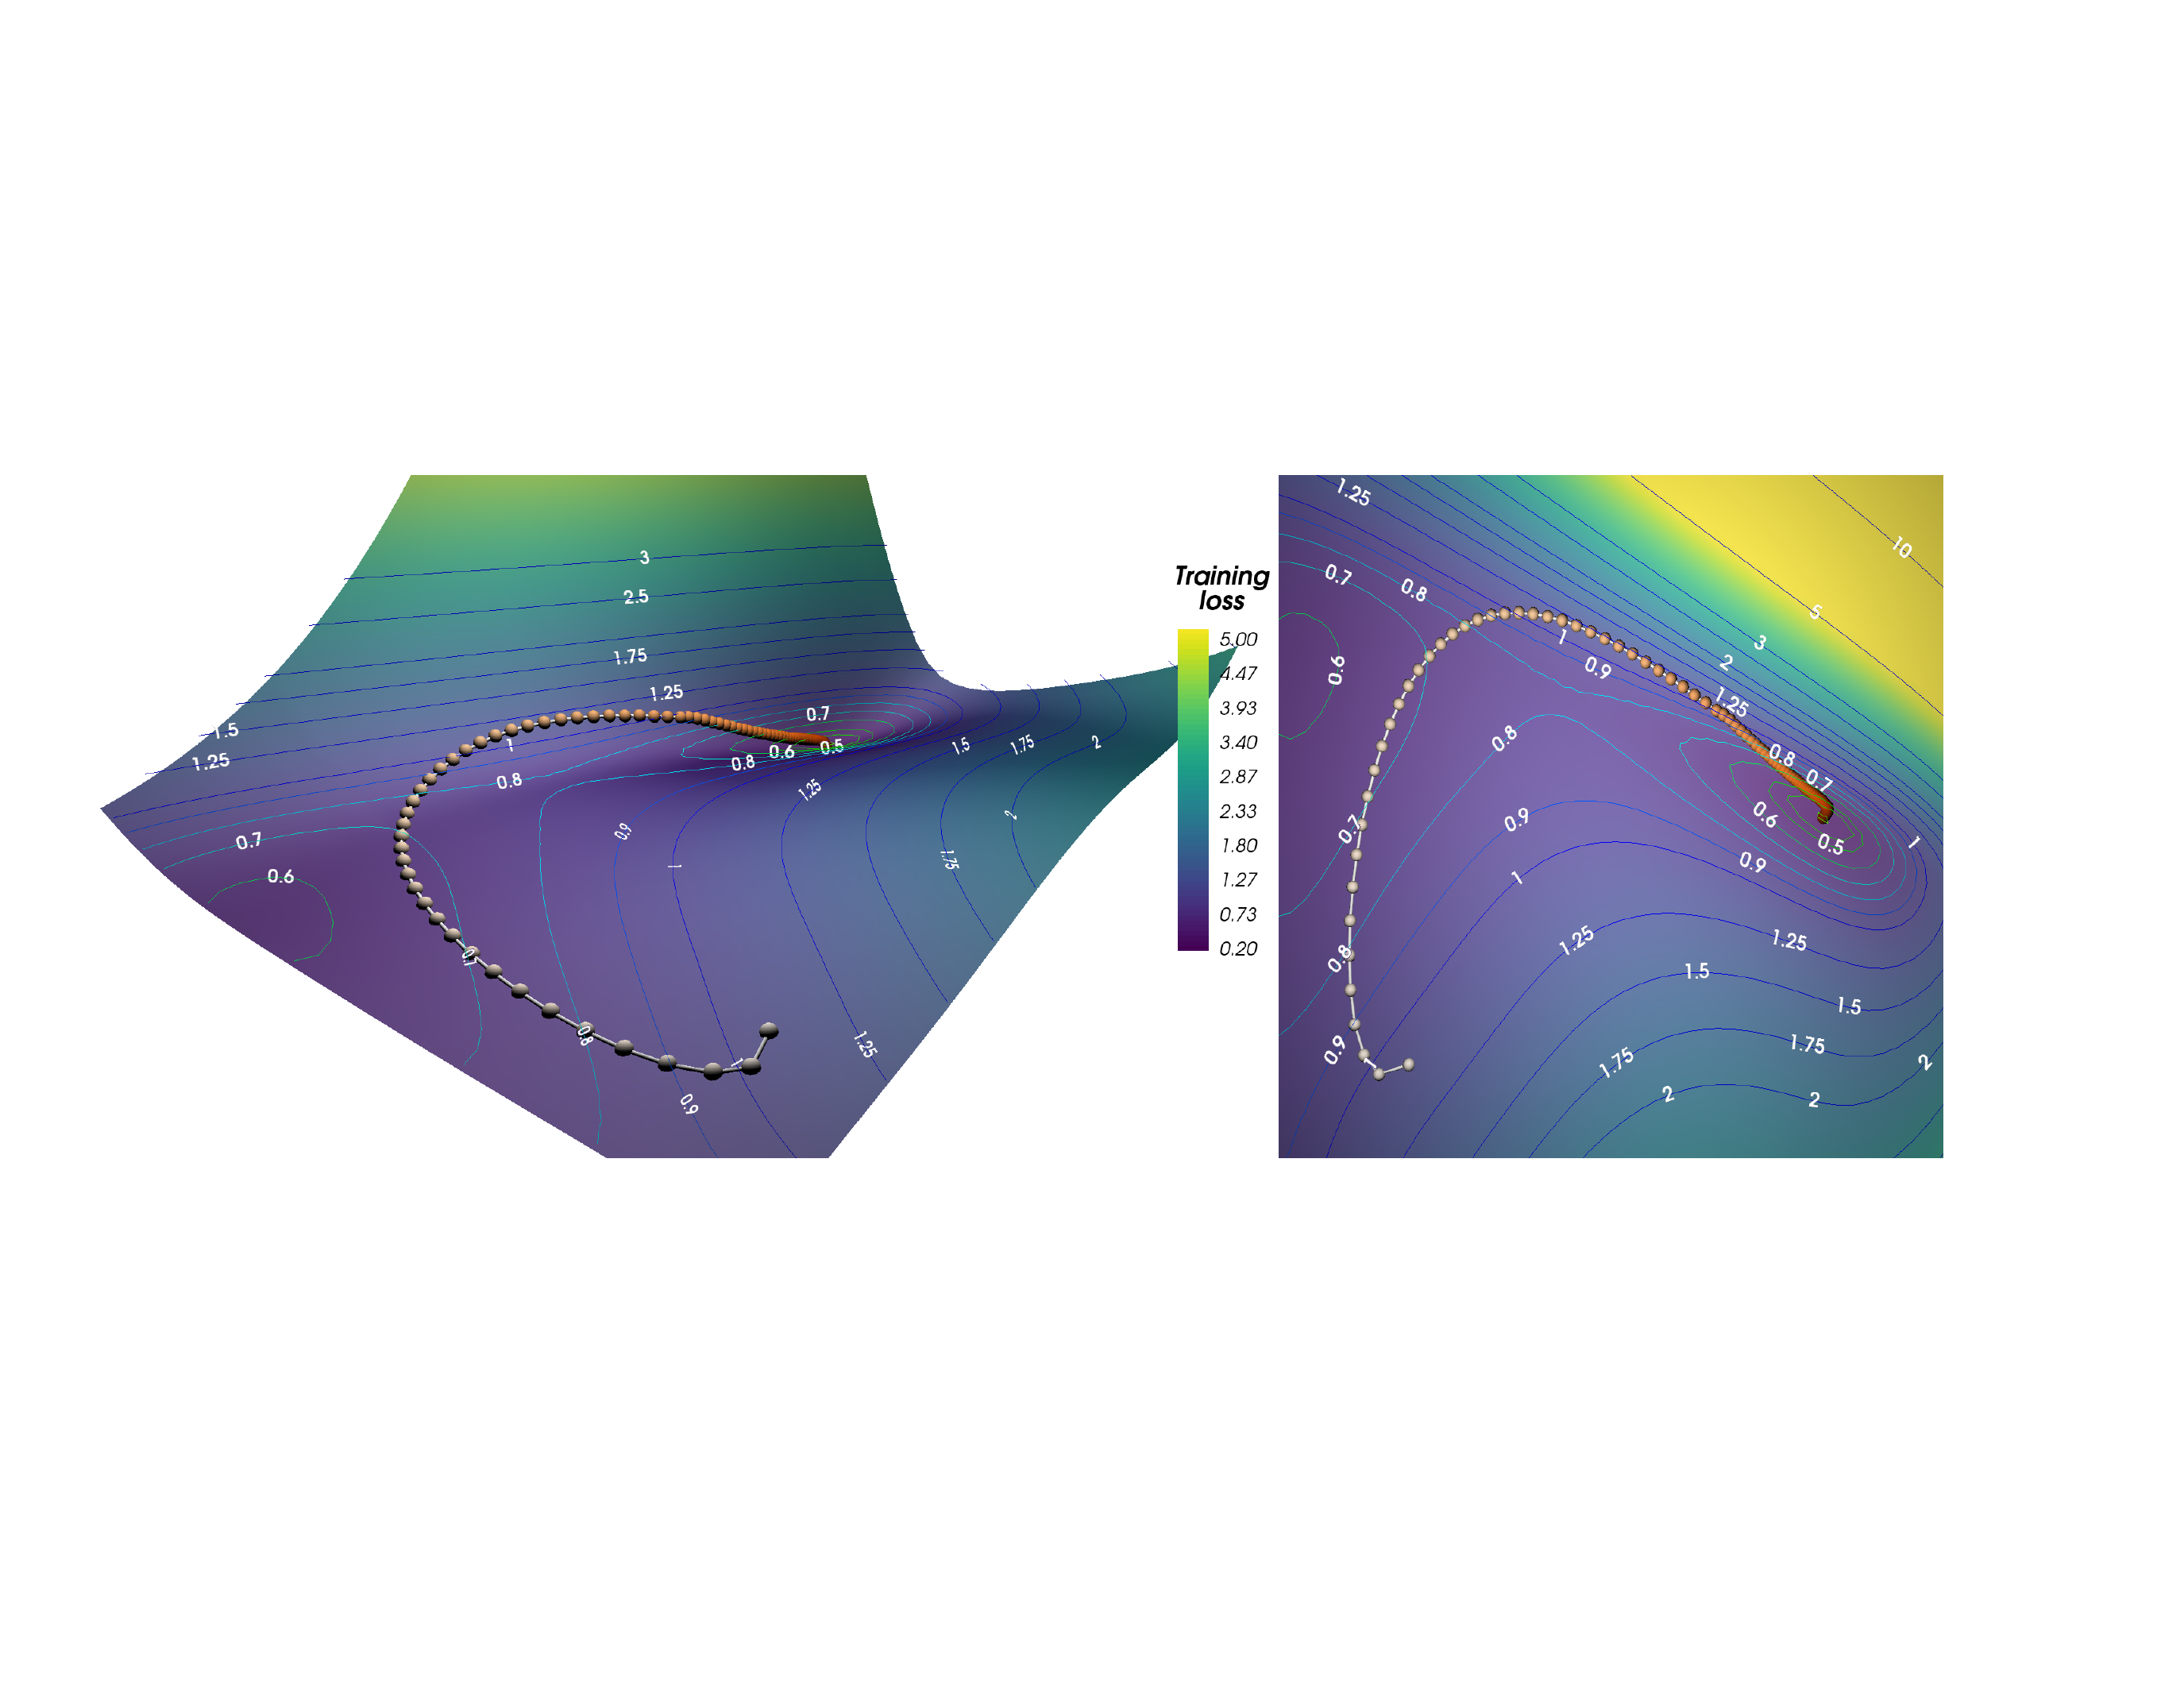} 
\includegraphics[width=0.99\linewidth]{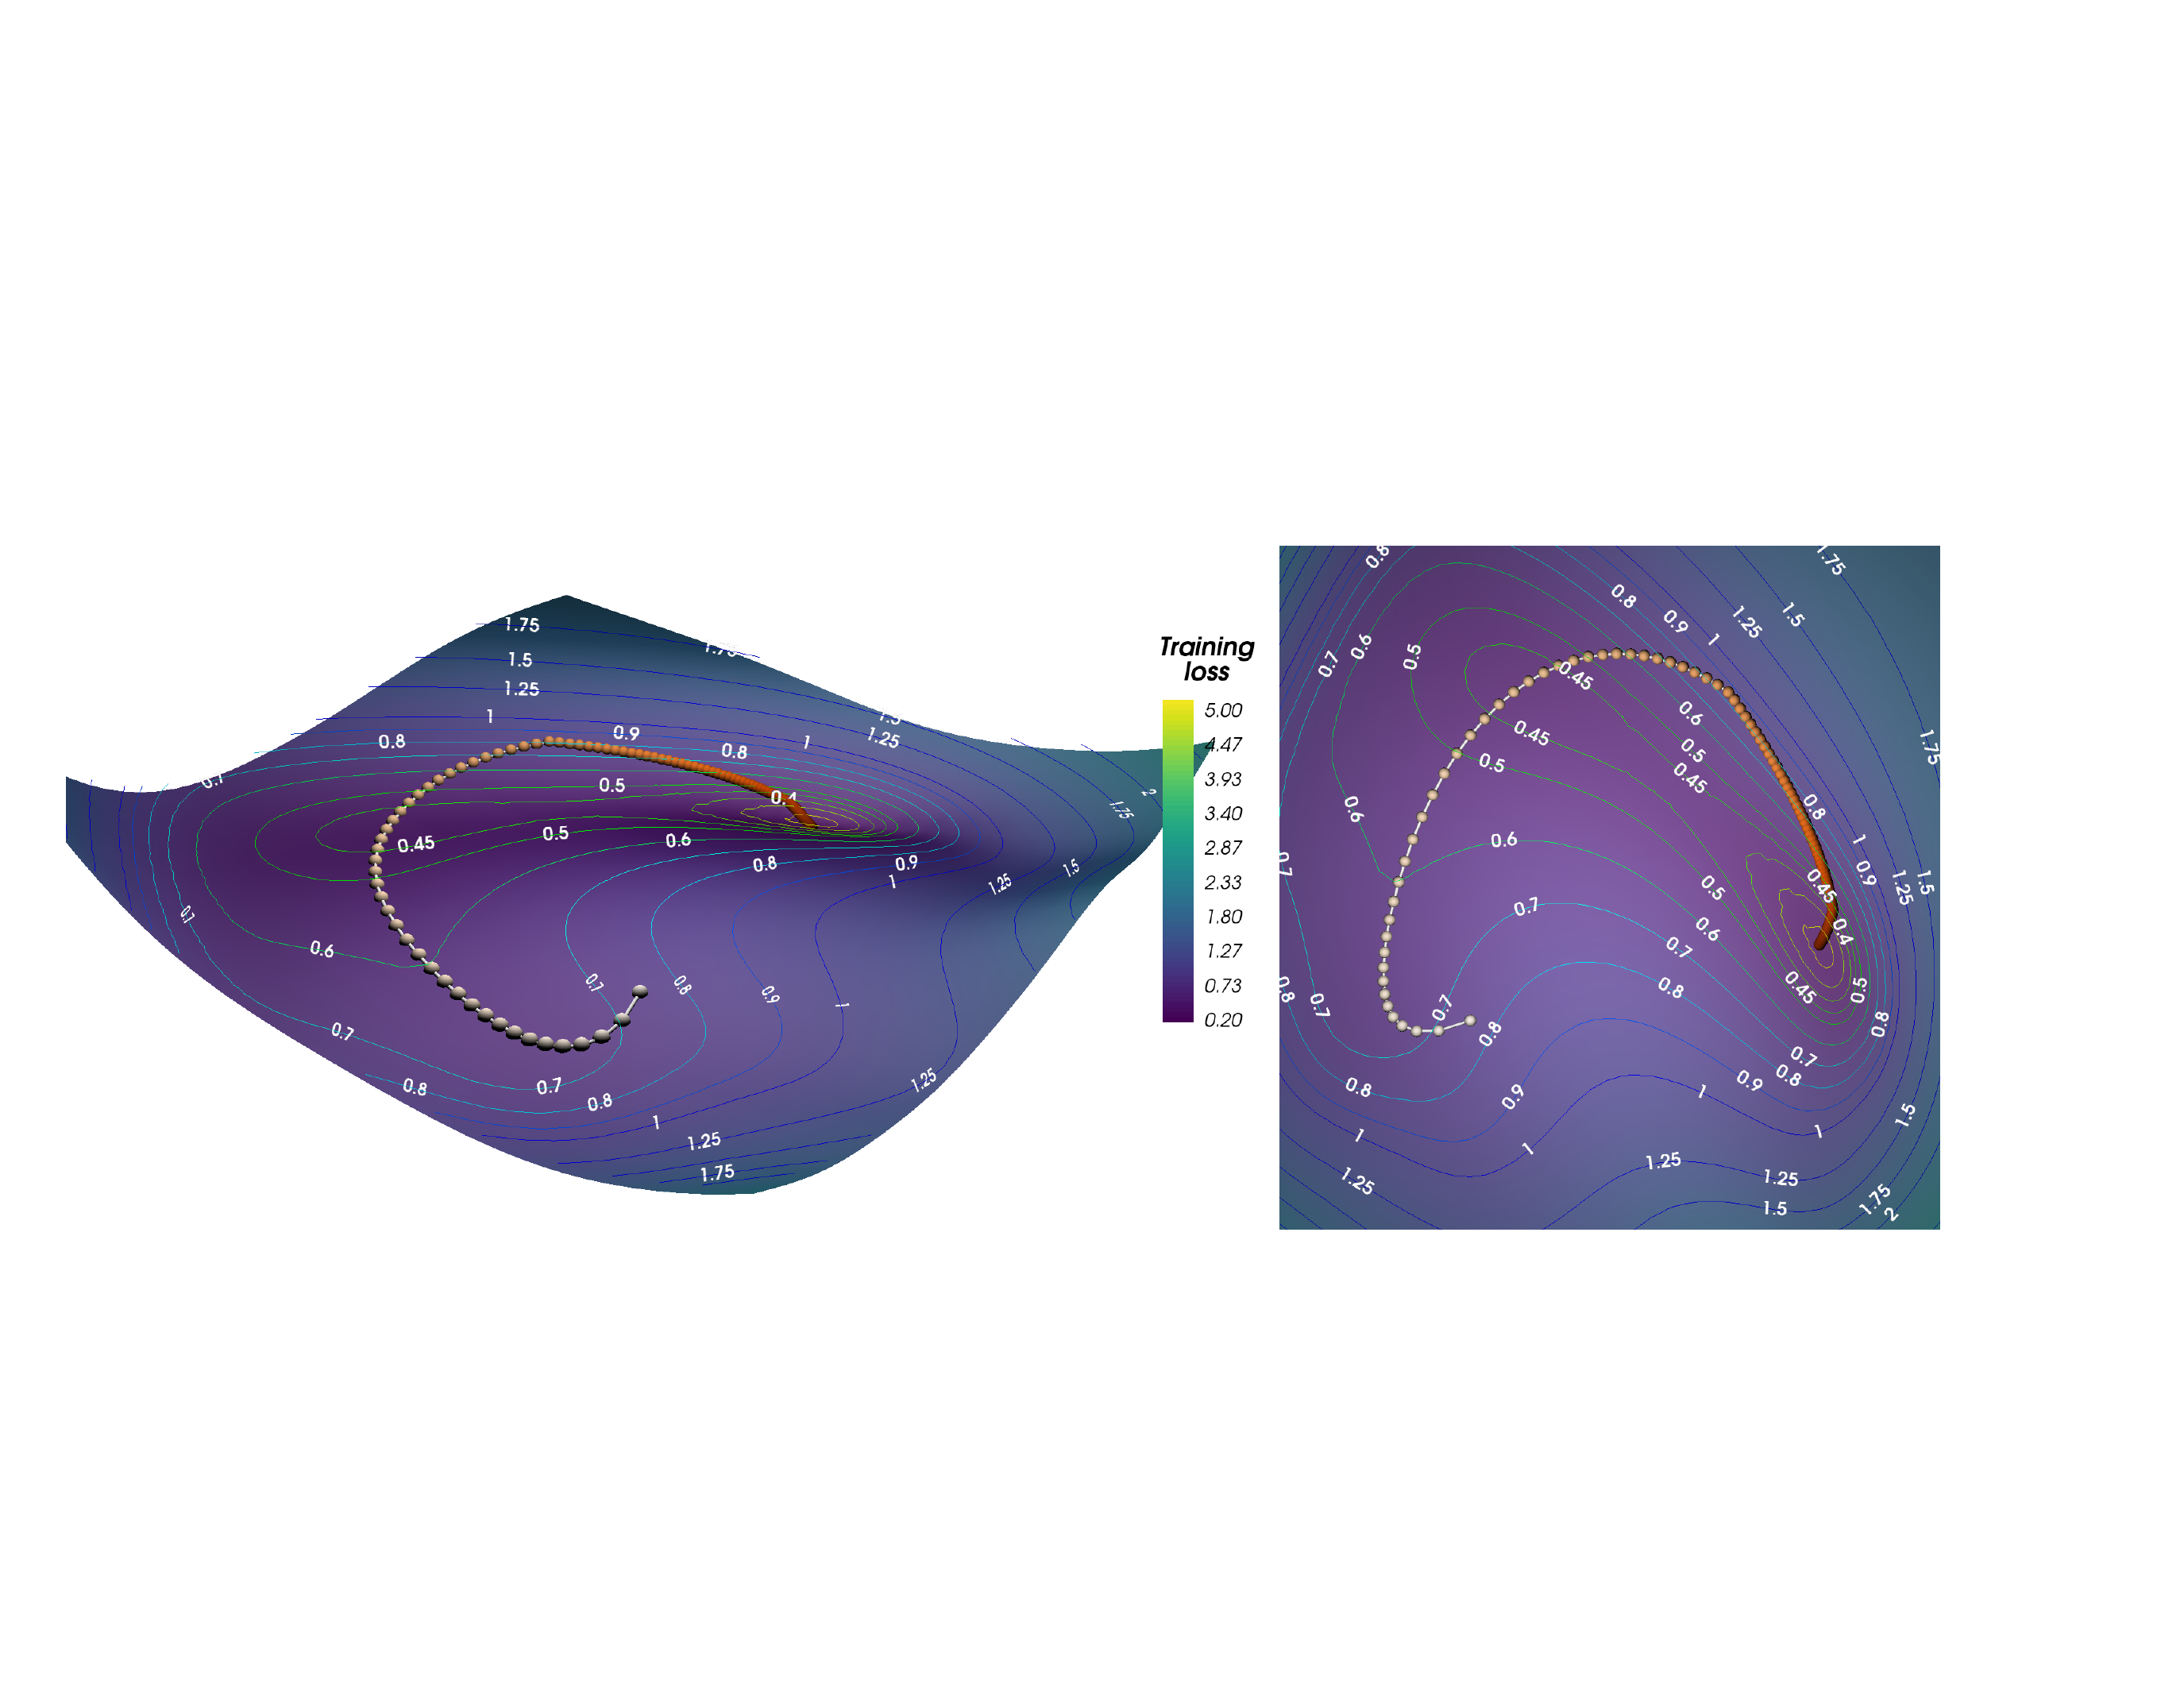}
\includegraphics[width=0.99\linewidth]{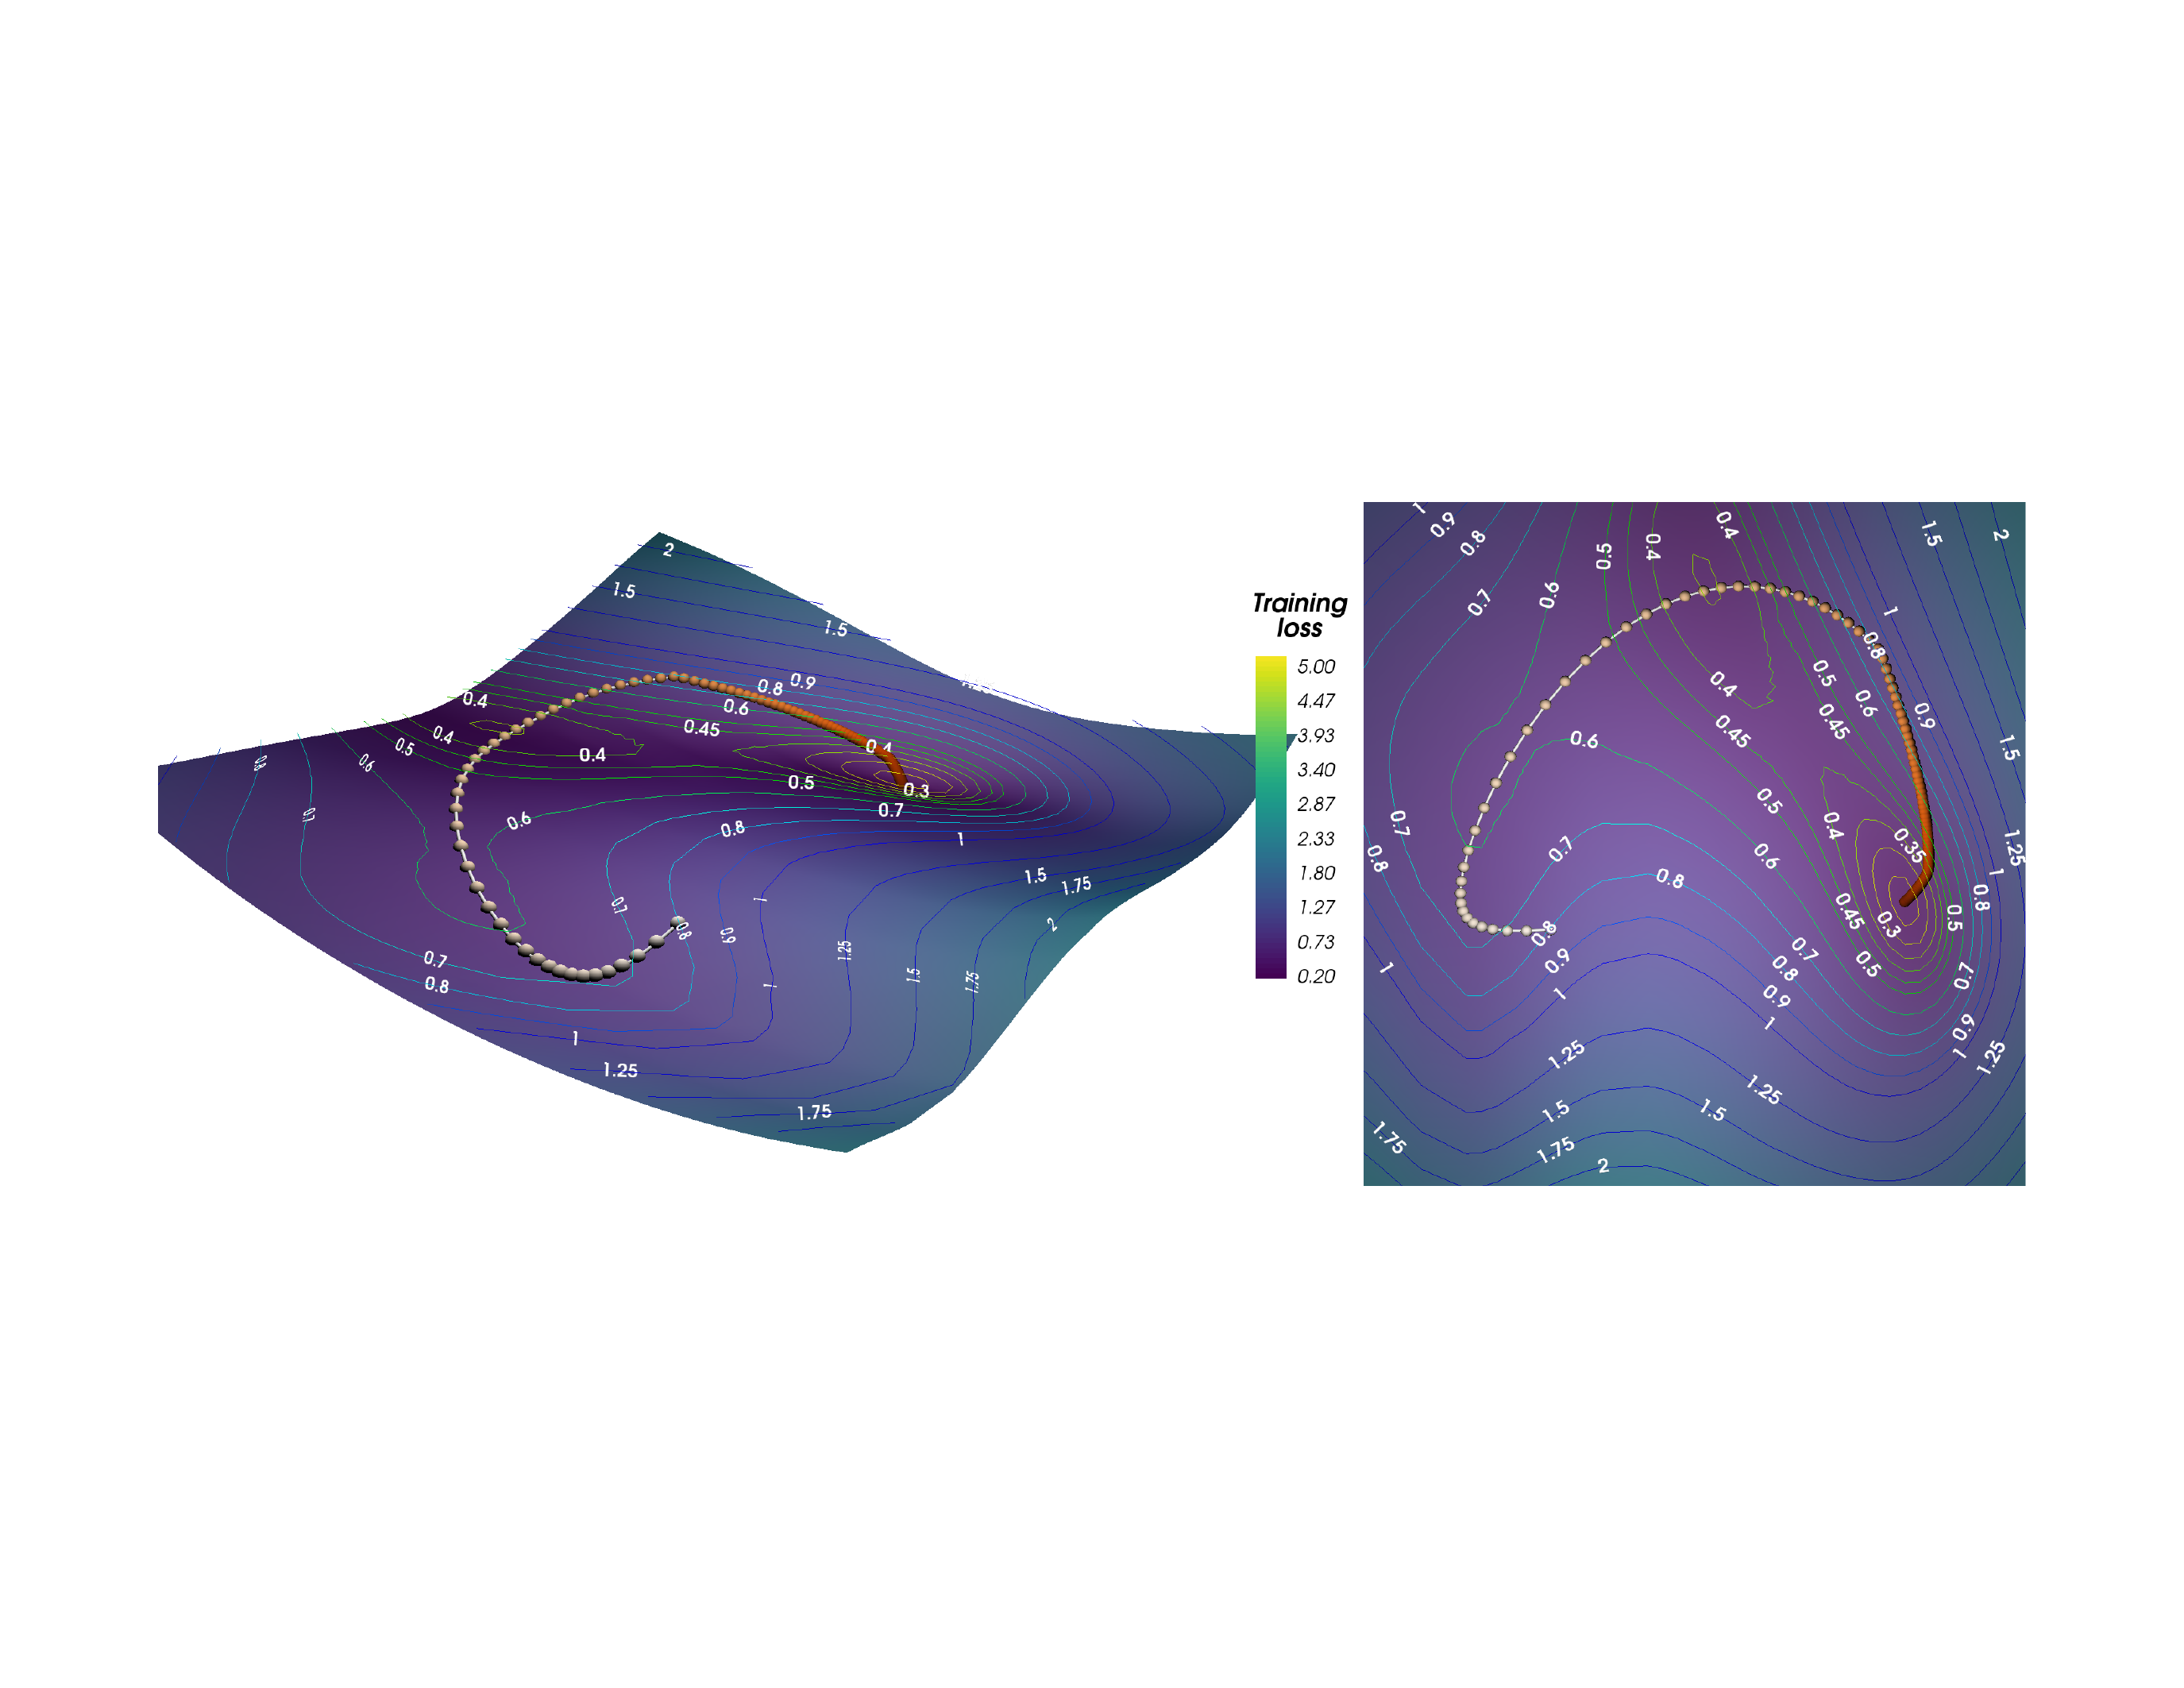} 
\caption{Loss landscapes of the considered architectures. Top: FNO, center: $\MFNO$, bottom: $\FNONeXt$ version 1\label{fig:landscapes}}
\end{figure}

These results allow us to make several observations. First, the FNO loss landscape exhibits much higher curvature than the other two architectures, which are both fairly flat in the vicinity of the found loss minimizer. Qualitatively, however, all landscapes exhibit the same pair of neighboring minima with a separating saddle point, which creates a curved loss valley. Further, the trajectories are surprisingly similar across architectures. In each case, the SGD-based optimization (Adam) procedures crossed the first minimum's basin before entering the second lower basin. Hence, the main difference between these different landscapes to explain the superior performance of $\FNONeXt$ appears to boil down to the depth of their respective loss minimum. 

To further investigate the observed similarities between training trajectories, we decided to compare them across additional PCA dimensions. The corresponding results are shown in a scatterplot matrix in \cref{fig:splom}.

\begin{figure}[h!]
\center
\includegraphics[width=0.99\linewidth]{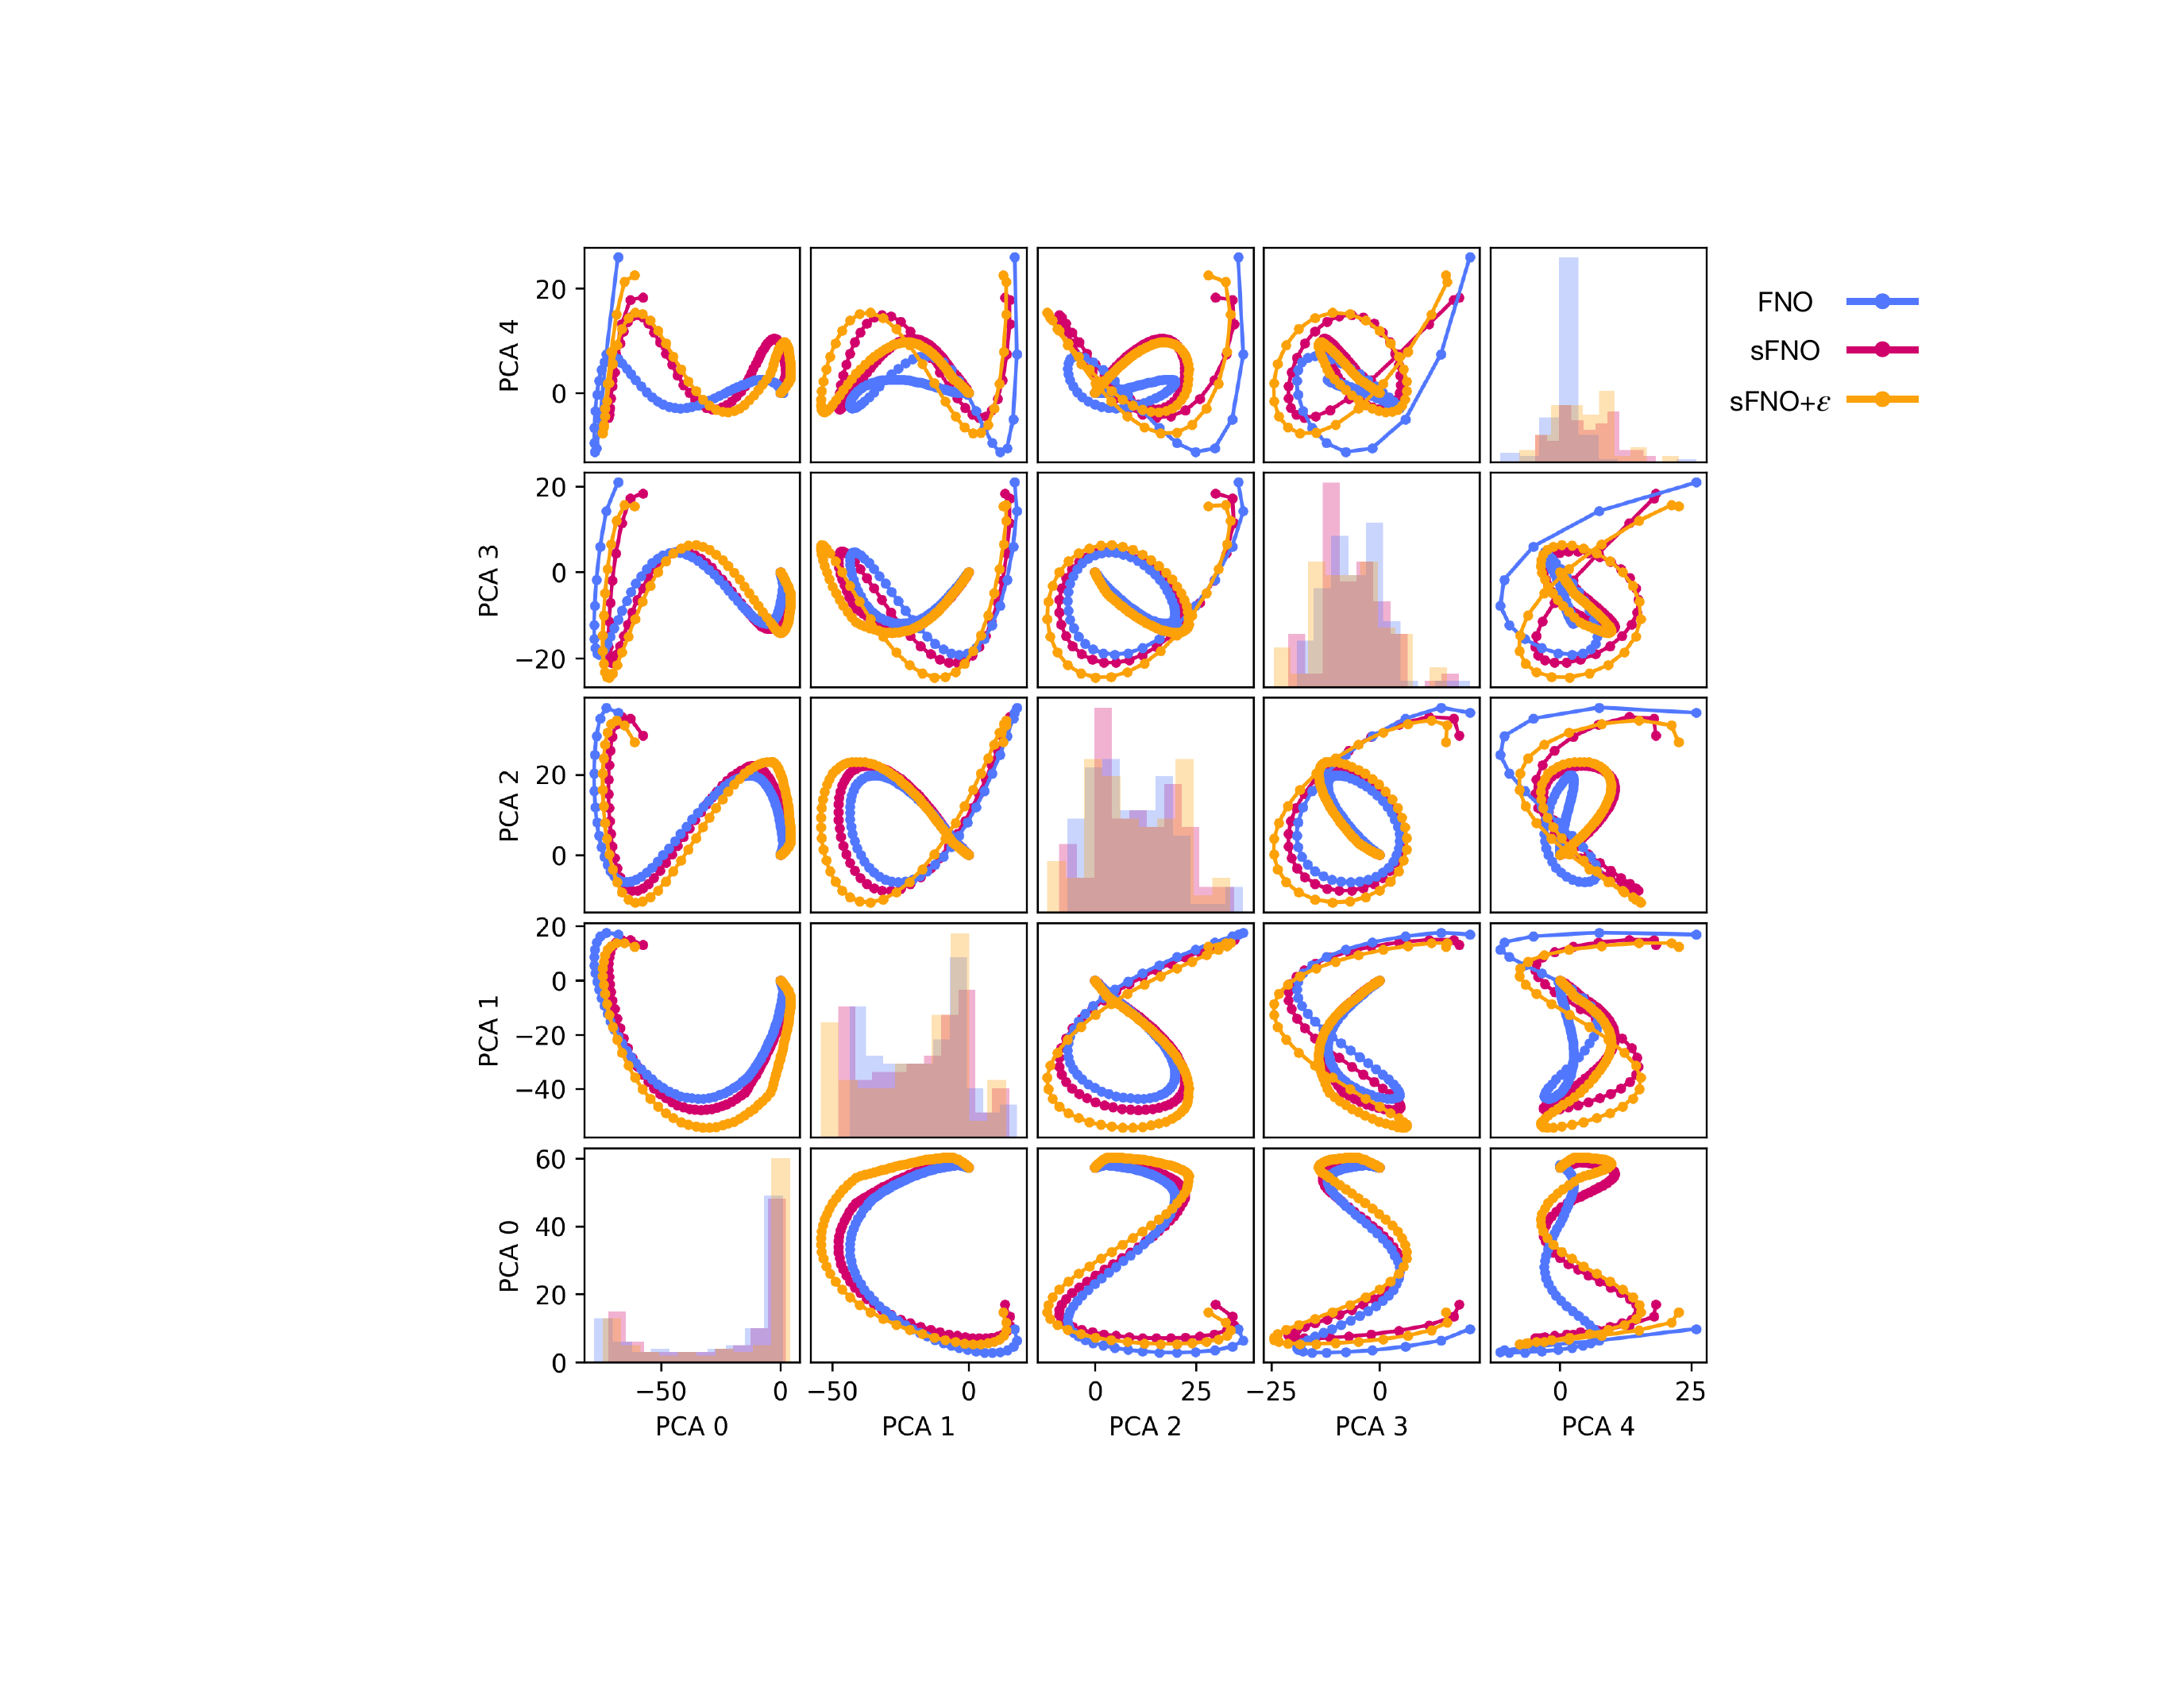}
\caption{Visual comparison of learning trajectories in PCA coordinates for FNO, $\MFNO$, and $\FNONeXt$ architectures. The first five principal components are considered. 
%Bluish: FNO, Redish: $\MFNO$, Gold: $\FNONeXt$
\label{fig:splom}}
\end{figure}

Note that the orientations of the principal components were matched using a simple geometric correlation criterion to facilitate comparison. This visualization confirms the remarkable qualitative similarities between the different architectures' learning trajectories. Nonetheless, these similarities decrease in higher dimensions. A possible interpretation of these observations is that the very low-dimensional nature of the parameter subspace in which the comparison is performed is too low to allow for a more insightful comparison between architectures. Alternatively, the linear nature of the dimensionality reduction may obfuscate the existence of a low-dimensional, nonlinear training trajectory manifold that more effectively captures the training dynamic. We intend to explore both avenues in future work. 

% {\color{red}{To add Xavier. A.}}
