# Supplementary material for: Out-of-distributional risk bounds for neural operators with applications to the Helmholtz equation
Source: arXiv:2301.11509 source file (2023-07-04)
Supplement: Supplementary file 3 [file 0.tex]

%%%%%%%%%%%%%%%%%%%%%%%%%%%%%%%%%%%%%%%%%%%%%%%%%%%%%%%%%%%%%%%%%

\section{Interpretation of the skip Connection} \label{NewtonMethod}
{\color{red}{it should be rewritten I think. A}}
We discuss the mathematical interpretation of our architecture %FNONeXt,
base on \citet{you2022learning}. 
We assume that forward or inverse problems in \ref{PDE1} and \ref{PDE2}) are translate into solving the following implicit equations:
\begin{align}
\mathcal{J}(m) = 0, \ \label{Implicit-equation}
\end{align}
where forward and inverse problems correspond to $m=u, a$, respectively. Both of forward and inverse problems can have implicit equations, for example, the mapping $\mathcal{J}$ in the forward and inverse problems can be applied as 
\begin{itemize}
\item (Forward problem) $\mathcal{J}(u):=\left( (\boldsymbol{\mathrm{L}}_{a}u-f) \bigr|_{D}, \boldsymbol{\mathcal{B}} u \right) \in \mathcal{U}(D; \mathbb{R}^{d_u})^{*}\times \mathcal{U}(\partial D; \mathbb{R}^{d_u})$
\item (Inverse problem) $\mathcal{J}(a):=\left\|\,u\bigr|_{\Sigma} - \boldsymbol{\mathrm{F}}(a)\, \right\|^{2}_{\mathcal{U}(\Sigma; \mathbb{R}^{d_u})} + \mathcal{R}(a) \in \mathbb{R}_{>0}$,
\end{itemize}
respectively, where $\boldsymbol{\mathrm{F}}: \mathcal{A}(D; \mathbb{R}^{d_a}) \to \mathcal{U}(\Sigma; \mathbb{R}^{d_u})$ is the forward operator mapping from the coefficient $a$ to the restricted solution $u\bigr|_{\Sigma}$ in (\ref{PDE1})--(\ref{PDE2}), and $\mathcal{R}(a)$ is some regularization term.
The problem (\ref{Implicit-equation}) is often solve by Newton's method \citep{Kaltenbacher, NakamuraPotthast, Bakushinsky}, that is, 
\begin{align}
m_{k+1}=m_{k}-s_{k}(\nabla \mathcal{J}(m_{k}))^{\dagger}\mathcal{J}(m_{k})=:m_{k}+ s_{k}\mathfrak{R}(m_{k}), \ \ k=0,1,..., \label{iterative solution}
\end{align}
where $m_{0}$ are some initial guesses, and $s_{k} \in \mathbb{R}$ is some step size. 
\par
Our proposed architecture can be interpreted as follows: $m_k$ and $m_{k+1}$ correspond to the input and output in one integral operator block, and $\mathfrak{R}(m_{k})$ corresponds to the composition of Fourier layer and MLPs, and $s_k$ corresponds to parameter multiplication. 
Adding $s_{k}\mathfrak{R}(u_{k})$ to $m_k$ corresponds to the skip-connection.
Layer normalization, drop-out, and stochastic depth are interpreted as playing a role to make training stable.
One integral operator block mimics one step of the Newton's iterative algorithm, and getting networks deeper indicates iteration step repeated many times.
It have been studied in \citet{you2022learning} that FNOs with skip-connection has universal approximation theorem (see Theorem 1 of \citet{you2022learning}) under the assumption that the fixed point for its implicit equation exists.
We expect that, by the same argument, our proposed architecture could also have the universal approximation. 
%The difference between \cite{you2022learning} and ours is that while the architecture in \cite{you2022learning} resembles ResNet in the sense of FNOs, ours does ConvNext, which is sophisticated ResNet along recent developments of Transformer. 
