# Supplementary material for: Out-of-distributional risk bounds for neural operators with applications to the Helmholtz equation
Source: arXiv:2301.11509 source file (2023-07-04)
Supplement: Supplementary file 6 [file 1.tex]

% ---------------------------
\subsection{Neural network reconstruction of the wavefield at $15$ Hz.}

\iffialse{
% ===============================================================
\section{Time-harmonic acoustic wave dataset}
\label{Euler_equation}
% ===============================================================

Our dataset corresponds to the propagation of waves 
associated with an acoustic medium characterized by
a wave speed. 
The waves, more precisely pressure field, are given 
at specific frequencies and known source.

% =======================================
\subsection{Time-harmonic wave equations}
% =======================================

We consider the propagation of time-harmonic acoustic 
waves for two dimensional domain $D \subset \mathbb{R}^2$.
The waves are given by the (scalar) pressure field $p$ 
and (vector) particle velocity $\boldsymbol{v}$ solutions 
to \citep{Faucher2020adjoint,martin2021time}
\begin{subequations} \label{eq:Euler} \begin{empheq}[left={\empheqlbrace}]{align}
  -\ii \omega \rho(\bx) \, \velocity(\bx,\omega) \,- \, 
   \nabla \pressure(\bx,\omega) \,=\, 0 \, , \quad \text{in $D$} \,, \\ 
  -\dfrac{\ii\omega}{\kappa(\bx)} \pressure(x,\omega) \,+\, \nabla \cdot \velocity(\bx,\omega) \,=\, f(\bx,\omega)\, , \quad \text{in $D$} \,,
\end{empheq} 
\end{subequations}
where $f$ is the time-harmonic source of angular 
frequency $\omega$, $\rho$ is the density and $\kappa$ 
the bulk modulus. The angular frequency is $\omega$.
The boundary of the domain $\partial D=\Gamma_1 \,\cup \,\Gamma_2$ 
is separated into two, following a geophysical configuration: a 
free-surface condition is imposed at the surface $\Gamma_1$ (that is
the interface between the medium and the air), while absorbing boundary
conditions \citep{engquist1977absorbing} are imposed elsewhere 
(that is, to truncate the numerical domain), see Figure~\ref{fig:boundary}. 
These correspond to conditions
\begin{subequations} \label{eq:time-harmonic:bc}  \begin{align}
\pressure(\bx,\omega) \,=\, 0\,, & \qquad \text{on $\Gamma_1$ (free surface),} \\
\partial_{\nu} \pressure(\bx,\omega) - \dfrac{i \omega}{c(\bx)} p(\bx,\omega) = 0\,, & \qquad \text{on $\Gamma_2$ (absorbing boundary conditions).}
\end{align}\end{subequations}

\begin{figure}[!ht] \centering
\begin{tikzpicture}[scale=1]
  \pgfmathsetmacro{\wid}{7.00} 
  \pgfmathsetmacro{\hei}{2.50}
  %% coordinates 
  \coordinate (r1)   at (  0.,  0.);  
  \coordinate (r2)   at (\wid,  0.);
  \coordinate (r3)   at (\wid,\hei); 
  \coordinate (r4)   at (  0.,\hei); 
  \draw[line width=2,\myblue]  (r4) to (r1) to (r2) to (r3);  
  \draw[line width=2,\myred]   (r3) to (r4);  
  \node[anchor=south east,\myred ,yshift=0mm,xshift=0.0em] at (r3) {$\Gamma_1$ (free surface)};
  \node[anchor=north east,\myblue,yshift=0mm,xshift=0.0em] at (r2) {$\Gamma_2$ (absorbing condition)};
  \node[anchor=south east,\myblue,yshift=0mm,xshift=0.0em, rotate=0] at (r1) {$\Gamma_2$};
  \node[anchor=south west,\myblue,yshift=0mm,xshift=0.0em, rotate=0] at (r2) {$\Gamma_2$};
  \node[anchor=south east,black  ,yshift=8mm,xshift=-5em, rotate=0] at (r2) {$D$};  

  \draw[mark=star,mark size=2.50,mark options={color=black,line width=0.75}] plot[] 
        coordinates{(.5*\wid,0.95*\hei)};
%%\draw[line width=1,densely dashed](0.0, 0.85*\hei) to (\wid, 0.85*\hei);  
\end{tikzpicture}
% =============================================================================

    \caption{Illustration of domain $D$: 
    free-surface condition is imposed on the the top (red line ,$\Gamma_1$),
    while absorbing absorbing boundary conditions are imposed elsewhere
    (blue line, $\Gamma_2$).
    The source (*) is typically positioned near surface.
    %  and the receivers (dashed line) slightly below.
    }
    \label{fig:boundary}
\end{figure}

Upon assuming constant density $\rho$, Problem~\eqref{eq:Euler} 
can be rewritten as the Helmholtz equation (see \citet[Remark~1]{faucher2020full}),
\begin{equation}
\label{eq:Helmholtz}
 -\bigg( \Delta \,+\, \dfrac{\omega^2}{c(\bx)^2} \bigg) \pressure(\bx,\omega)
    \,=\, -\mathrm{i}\omega\rho \, f(\bx,\omega)\,,
\end{equation}
where $c$ is the wave speed defined such that
\begin{equation}
  c(\bx) = \sqrt{\dfrac{\kappa(\bx)}{\rho(\bx)}} \, .
\end{equation}

% ===========================================================
\subsection{Dataset} \label{dataset:Helmholtz}
% ===========================================================

The dataset corresponds to the $N$ couples made up of a wave speed
and pressure field, $(c_k,p_k)_{k=1,\ldots,N}$, where $p_k$ solves 
\cref{eq:Helmholtz} using wave speed $c_k$. 
The sources $f$ in \cref{eq:Helmholtz} is taken a delta-Dirac function 
$\delta$, and we proceed as follow,
\begin{enumerate}
  \item Setup the geometrical domain $D$ and 
        configuration (i.e., dimension, frequency 
        for propagation, source position);
  \item Create a set of wave speeds that are independent 
        and identically distributed random variables,
        see~\cref{subsection:GRF-wavespeed};
  \item Solve the wave equation~\cref{eq:Helmholtz} on $D$
        for each wave speed $c_k$.
        Here, we use a \textit{Hybridizable Discontinuous Galerkin Method} 
        (HDG, \cite{Faucher2020adjoint}) for the discretization and (open-source) 
        software \texttt{hawen}, see \citet{faucher2021hawen}. 
  \item Save the resulting pressure field on a Cartesian grid.
\end{enumerate}
We further consider two experiments, each with different size 
of domain, position of sources, and where we impose different 
lower and upper bounds for the variation of the wave speeds.
}\fi

% ===========================================================
\subsection{Generation of data from the numerical perspective: HDG}
% ===========================================================

Accuracy of the discretization method for PDE is studied in literature, for instance \cite{griesmaier2011error} for HDG.
Roughly speaking, the accuracy of the PDE solver requires
to have a sufficient number of degrees of freedom per wavelength. 
In our simulations, we have at least 20 (usually it is assumed that 8 points per wavelength are sufficient). 

\begin{enumerate}
    \item We use an unstructured triangle mesh with about \num{25000} elements. This guarantees to have 
            enough degrees of freedom per wavelength. Another important aspect is the 
            accurate representation of the wave speed model. One main advantage of 
            software \texttt{hawen} is \textbf{not} to rely on a piecewise-constant
            representation. Namely, the wave speed model is allowed to vary within 
            each cell, to ensure that the representation captures all of the details.
            For an illustration, we refer to \cite[Figure 7]{Faucher2020adjoint}.
    \item  In addition to using sufficient degrees of freedom per wavelength and representation 
 that varies within each element of the mesh to ensure the accuracy, we can illustrate 
 in Figure~\ref{figure:wavefields} the accuracy by comparing the simulations performed
 on two different meshes: the one with \num{25000} elements which is used to generate
 the training set, and one with \num{50000} elements. We see 
 that  the relative error is in the magnitude of \num{e-6}.
\end{enumerate}
%%%%%%%%%%%%%%%%%

\setlength{\modelwidth}{4cm}
\setlength{\modelheight}{4cm}

\begin{figure}[ht!]\centering
\renewcommand{\modelfile}{Figures/accuracy_HDG/wavefield_mesh25k_scale1-1}
\subfigure[Wavefield solution on a mesh with about \num{25000} elements (used for the training data).]
          {\makebox[.28\linewidth][c]{{\input{Figures/accuracy_HDG/skeleton-wave}}}} \hspace*{1em}
\renewcommand{\modelfile}{Figures/accuracy_HDG/wavefield_mesh50k_scale1-1}
\subfigure[Wavefield solution on a mesh with about \num{50000} elements.]
          {\makebox[.28\linewidth][c]{{\input{Figures/accuracy_HDG/skeleton-wave}}}} \hspace*{1em}
\renewcommand{\modelfile}{Figures/accuracy_HDG/relative-error_logscale_-5_-2}
\subfigure[Relative difference.]
          {\makebox[.28\linewidth][c]{{\input{Figures/accuracy_HDG/skeleton-error}}}}
\caption{Illustration of the accuracy of the computations with the direct wave solver.}
\label{figure:wavefields}
\end{figure}

% ===========================================================
\subsection{Experimental dataset}
% ===========================================================

We consider two datasets. For the first experiment, 
we have the following setup: 
%\begin{subequations}\begin{empheq}[left={\text{Experiment 1} \,\empheqlbrace\quad}]{align}
\begin{equation}\label{experiment1}
\text{Experiment 1} \,\left\lbrace\quad\begin{aligned}
 & \text{2D domain of size \num{3.81}$\times$\num{3.81}\si{\km\squared}} \\
 & \text{\num{40000} GRF wave speeds generated, imposing \,
         $\num{1.5}\si{\km\per\second}\,\leq c(x) \leq \num{3}\si{\km\per\second}$} \\
 & \text{The data are $p$ that solve 
         \cref{eq:Euler} at frequency $\omega/(2\pi)=$ \num{7}\si{\Hz} (one field per wave speed)}.
\end{aligned}\right.\end{equation}
%\end{empheq}\end{subequations}
Both the wave speeds and the pressure field solution are 
represented on a Cartesian grid of size \num{128}$\times$\num{128}
pixels, that is, using a grid step of \num{30}\si{\meter}.
We illustrate in \cref{figure:cp-GRF:experiment1} a realization of 
the wave speed model and the corresponding pressure field.

% ---------------------------
\setlength{\modelwidth} {5cm}
\setlength{\modelheight}{5cm}
% ---------------------------
\begin{figure}[h!]\centering
\subfigure[GRF realization of wave speed model $c$.]{
\renewcommand{\modelfile}{Figures/dataset/GRF/experiment1_cp_scale1500to3000}
  \pgfmathsetmacro{\cmin}{1.50}
  \pgfmathsetmacro{\cmax}{3.00}
  \pgfmathsetmacro{\xmin}{0}
  \pgfmathsetmacro{\xmax}{3.810}
  \pgfmathsetmacro{\zmin}{0}
  \pgfmathsetmacro{\zmax}{3.810}
{\input{./Figures/dataset/GRF/skeleton-cp}}
}
\begin{tikzpicture}[scale=1]
\draw[line width=2,black,->]  (1.50,0) to node[draw,rectangle,black,anchor=south,text width=7em,align=center,line width=1pt,yshift=0.50em]{from $c$ to $\pressure$ solving \eqref{eq:Euler}} (4.4,0);  
\end{tikzpicture}
\subfigure[Real part of the pressure field at 7 \si{\Hz} frequency.]{
\renewcommand{\modelfile}{Figures/dataset/GRF/experiment1_p_scale1e-1_real_bluered}
  \pgfmathsetmacro{\xmin}{0}
  \pgfmathsetmacro{\xmax}{3.810}
  \pgfmathsetmacro{\zmin}{0}
  \pgfmathsetmacro{\zmax}{3.810}
  \pgfmathsetmacro{\cmin}{-0.1}
  \pgfmathsetmacro{\cmax}{0.1}
{\input{./Figures/dataset/GRF/skeleton-wave}}
}
\caption{Illustration of the full-wave dataset for Experiment~1
         that considers a computational domain of size 
         \num{3.81}$\times$\num{3.81}\si{\km\squared} 
         with a source buried in the domain.
         The wave speed and pressure field are represented 
         on a Cartesian grid of size \num{128}$\times$\num{128}
         with a grid step of \num{30}\si{\meter}.
         The complete dataset corresponds to \num{40000} couples
         made up of a wave speed model and associated acoustic 
         wave.}
\label{figure:cp-GRF:experiment1}
\end{figure}

For the second experiment, we consider a smaller domain 
but higher variation of wave speed, and the source is 
positioned near surface such that:
%\begin{subequations}\begin{empheq}[left={\text{Experiment 1} \,\empheqlbrace\quad}]{align}
\begin{equation}\label{experiment2}
\text{Experiment 2} \,\left\lbrace\quad\begin{aligned}
 & \text{2D domain of size \num{1.27}$\times$\num{1.27}\si{\km\squared}} \\
 & \text{\num{40000} GRF wave speeds generated, imposing \,
         $\num{1.5}\si{\km\per\second}\,\leq c(x) \leq \num{5}\si{\km\per\second}$} \\
 & \text{The data are $p$ that solve 
         \cref{eq:Euler} at frequency $\omega/(2\pi)=$ \num{12} and \num{15} \si{\Hz}}.
\end{aligned}\right.\end{equation}
%\end{empheq}\end{subequations}
Both the wave speeds and the pressure field solution are 
represented on a Cartesian grid of size \num{64}$\times$\num{64}
pixels, that is, using a grid step of \num{20}\si{\meter}.
We illustrate in \cref{figure:cp-GRF:experiment2} a wave speed
model and the corresponding pressure field.

% ---------------------------
\setlength{\modelwidth} {5cm}
\setlength{\modelheight}{5cm}
% ---------------------------
\begin{figure}[h!]\centering
\subfigure[GRF realization of wave speed model $c$.]{
\renewcommand{\modelfile}{Figures/dataset/GRF/cp_128x128_00001}
  \pgfmathsetmacro{\cmin}{1.50}
  \pgfmathsetmacro{\cmax}{5.00}
  \pgfmathsetmacro{\xmin}{0}
  \pgfmathsetmacro{\xmax}{1.270}
  \pgfmathsetmacro{\zmin}{0}
  \pgfmathsetmacro{\zmax}{1.270}
{\input{./Figures/dataset/GRF/skeleton-cp}}
}
\begin{tikzpicture}[scale=1]
\draw[line width=2,black,->]  (1.50,0) to node[draw,rectangle,black,anchor=south,text width=7em,align=center,line width=1pt,yshift=0.50em]{from $c$ to $\pressure$ solving \eqref{eq:Euler}} (4.4,0);  
\end{tikzpicture}
\subfigure[Real part of the pressure field at 12 \si{\Hz} frequency.]{
\renewcommand{\modelfile}{Figures/dataset/GRF/wavefield-p_cp00001_12Hz_scale5e-2_real_bluered}
  \pgfmathsetmacro{\xmin}{0}
  \pgfmathsetmacro{\xmax}{1.270}
  \pgfmathsetmacro{\zmin}{0}
  \pgfmathsetmacro{\zmax}{1.270}
  \pgfmathsetmacro{\cmin}{-0.05}
  \pgfmathsetmacro{\cmax}{0.05}
{\input{./Figures/dataset/GRF/skeleton-wave}}
}
\caption{Illustration of the full-wave dataset for Experiment~2
         that considers a computational domain of size 
         \num{1.27}$\times$\num{1.27}\si{\km\squared} with
         a source near surface.
         The wave speed and pressure field are represented 
         on a Cartesian grid of size \num{64}$\times$\num{64}
         with a grid step of \num{20}\si{\meter}. 
         The complete dataset corresponds to \num{40000} couples
         made up of a wave speed model and associated acoustic 
         wave.}
\label{figure:cp-GRF:experiment2}
\end{figure}

%% ---------------------------
%\setlength{\modelwidth} {5cm}
%\setlength{\modelheight}{5cm}
%% ---------------------------
%\begin{figure}[ht!]\centering
%  \renewcommand{\modelfile}{Figures/dataset/GRF/cp_128x128_00001}
%  \subfloat[][GRF realization of wave speed model $c$ represented
%              on a \num{128}$\times$\num{128} grid.]
%             {\input{./Figures/dataset/GRF/skeleton-cp}}
%  \renewcommand{\modelfile}{Figures/dataset/GRF/wavefield-p_cp00001_12Hz_scale5e-2_real}
%  \subfloat[][Real part of the pressure field at 12 \si{\Hz} 
%              frequency for a source positioned in $(610,10)$ 
%              \si{m} represented on a \num{64}$\times$\num{64} grid.]
%             {\input{./Figures/dataset/GRF/skeleton-wave}}
%
%\vspace*{-12em}
%\begin{tikzpicture}[scale=1]
%\draw[line width=2,black,->]  (1.50,0) to node[draw,rectangle,black,anchor=south,text width=7em,align=center,line width=1pt,yshift=0.50em]{from $c$ to $\pressure$ solving \eqref{eq:Euler}} (4.4,0);  
%
%\end{tikzpicture}
%\vspace*{8.00em}
%
%  \caption{Illustration of the full-wave dataset.}
%  \label{figure:cp-GRF}
%\end{figure}
