# Supplementary material for: Out-of-distributional risk bounds for neural operators with applications to the Helmholtz equation
Source: arXiv:2301.11509 source file (2023-07-04)
Supplement: Supplementary file 7 [file 2.tex]

We empirically analyze generalization \emph{out-of-distribution of the network}. A detailed explanation of the parameters of the dataset is presented in \cref{Out-of-distribution}. See \cref{fig:OOD_reconstruction_w_annotations} for a visualization of an anisotropic case (all networks are trained with isotropic covariance).
\setlength{\modelwidth} {4.cm}
\setlength{\modelheight}{4.cm}
\begin{figure}[!ht] \centering
   \input{Figures/OOD_main_paper/set5/skeleton_online_set5}
    \vspace*{-1em}
    \label{fig:OOD_reconstruction_w_annotations}
    \caption{OOD (family 6) analysis of set $6$, anisotropic case, see table \cref{table:ood} and \cref{OOD:6}.}
\end{figure}
