# Supplementary material for: Out-of-distributional risk bounds for neural operators with applications to the Helmholtz equation
Source: arXiv:2301.11509 source file (2023-07-04)
Supplement: Supplementary file 8 [file tableofNotation.tex]

%%%%%%%%%%%%%%%%%%%%%%%%%%%%%%%%%%%%
